# Supplementary material for: QMamba: Post-Training Quantization for Vision State Space Models
Source: arXiv:2501.13624 source file (2025-01-23)
Supplement: Supplementary file 1 [file outlier.tex]

\section{Additional Analysis on OMSE Initialization}
\label{outlier}

\begin{figure}[tp]
  \centering
  \subcaptionbox{Observation on SSMs of Vim-S\label{outlier:box}}{
    \includegraphics[width=0.485\linewidth]{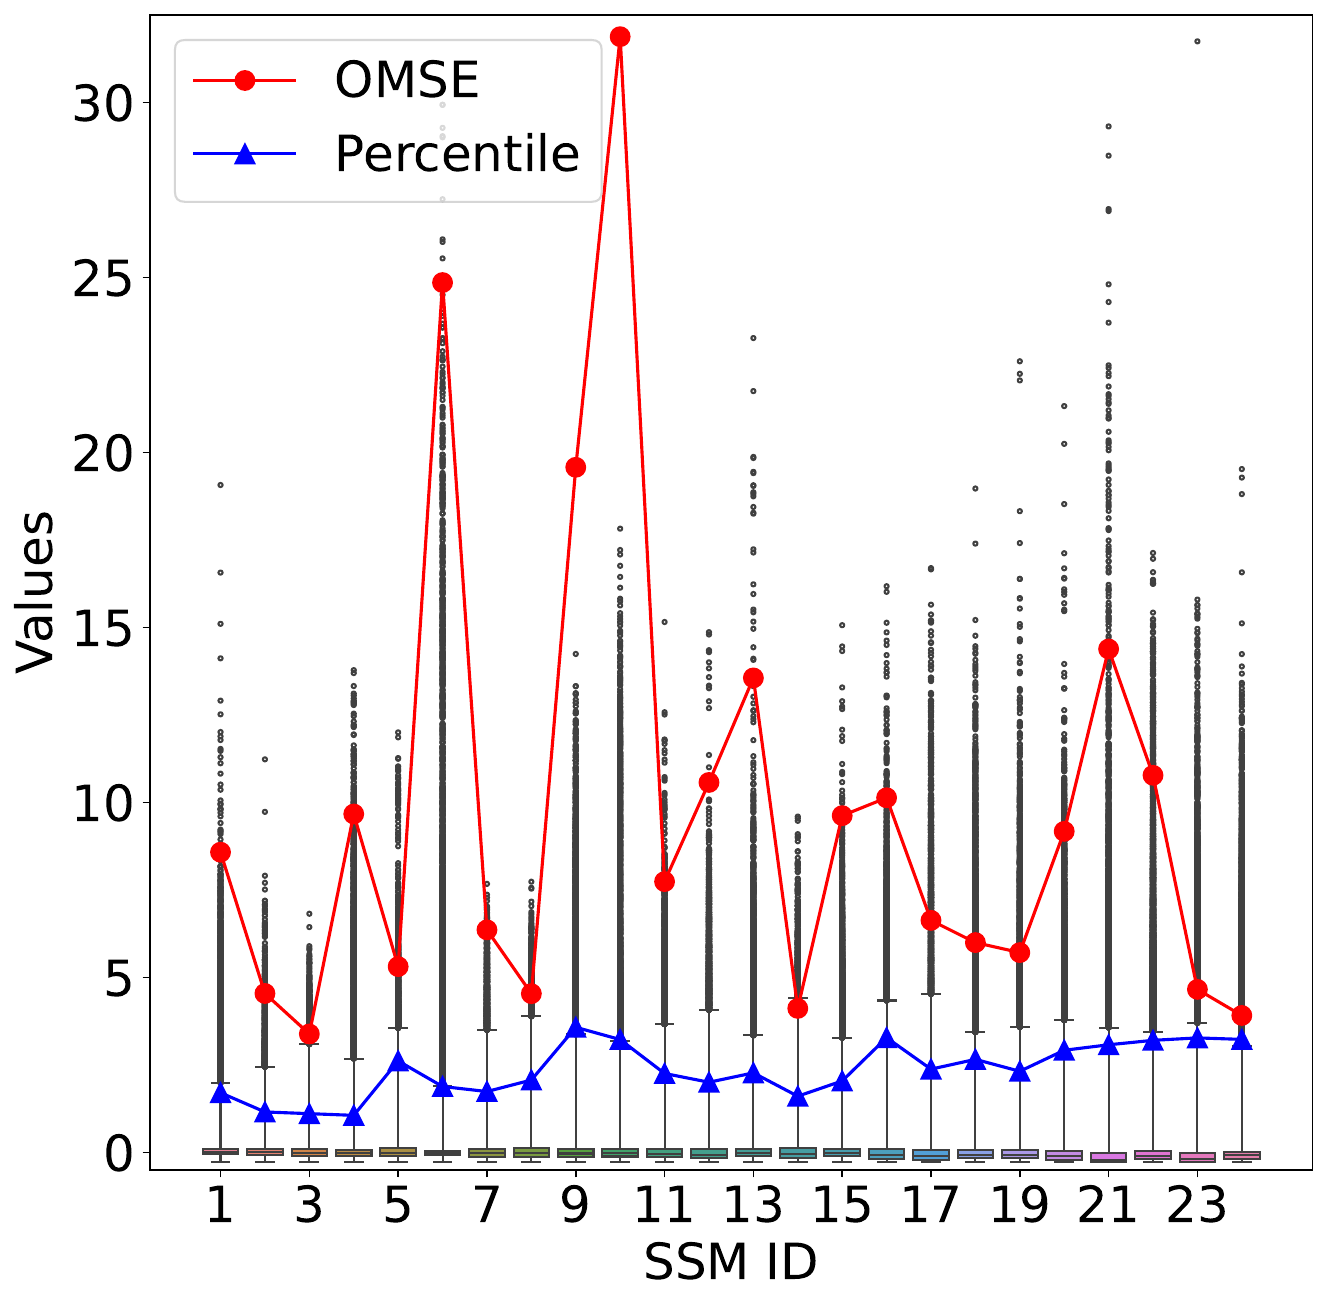}%0.342
  }\hfill %\hspace{0.01\textwidth}
  \subcaptionbox{Observation on the 5-th SSM\label{outlier:hist}}{
    \includegraphics[width=0.48\linewidth]{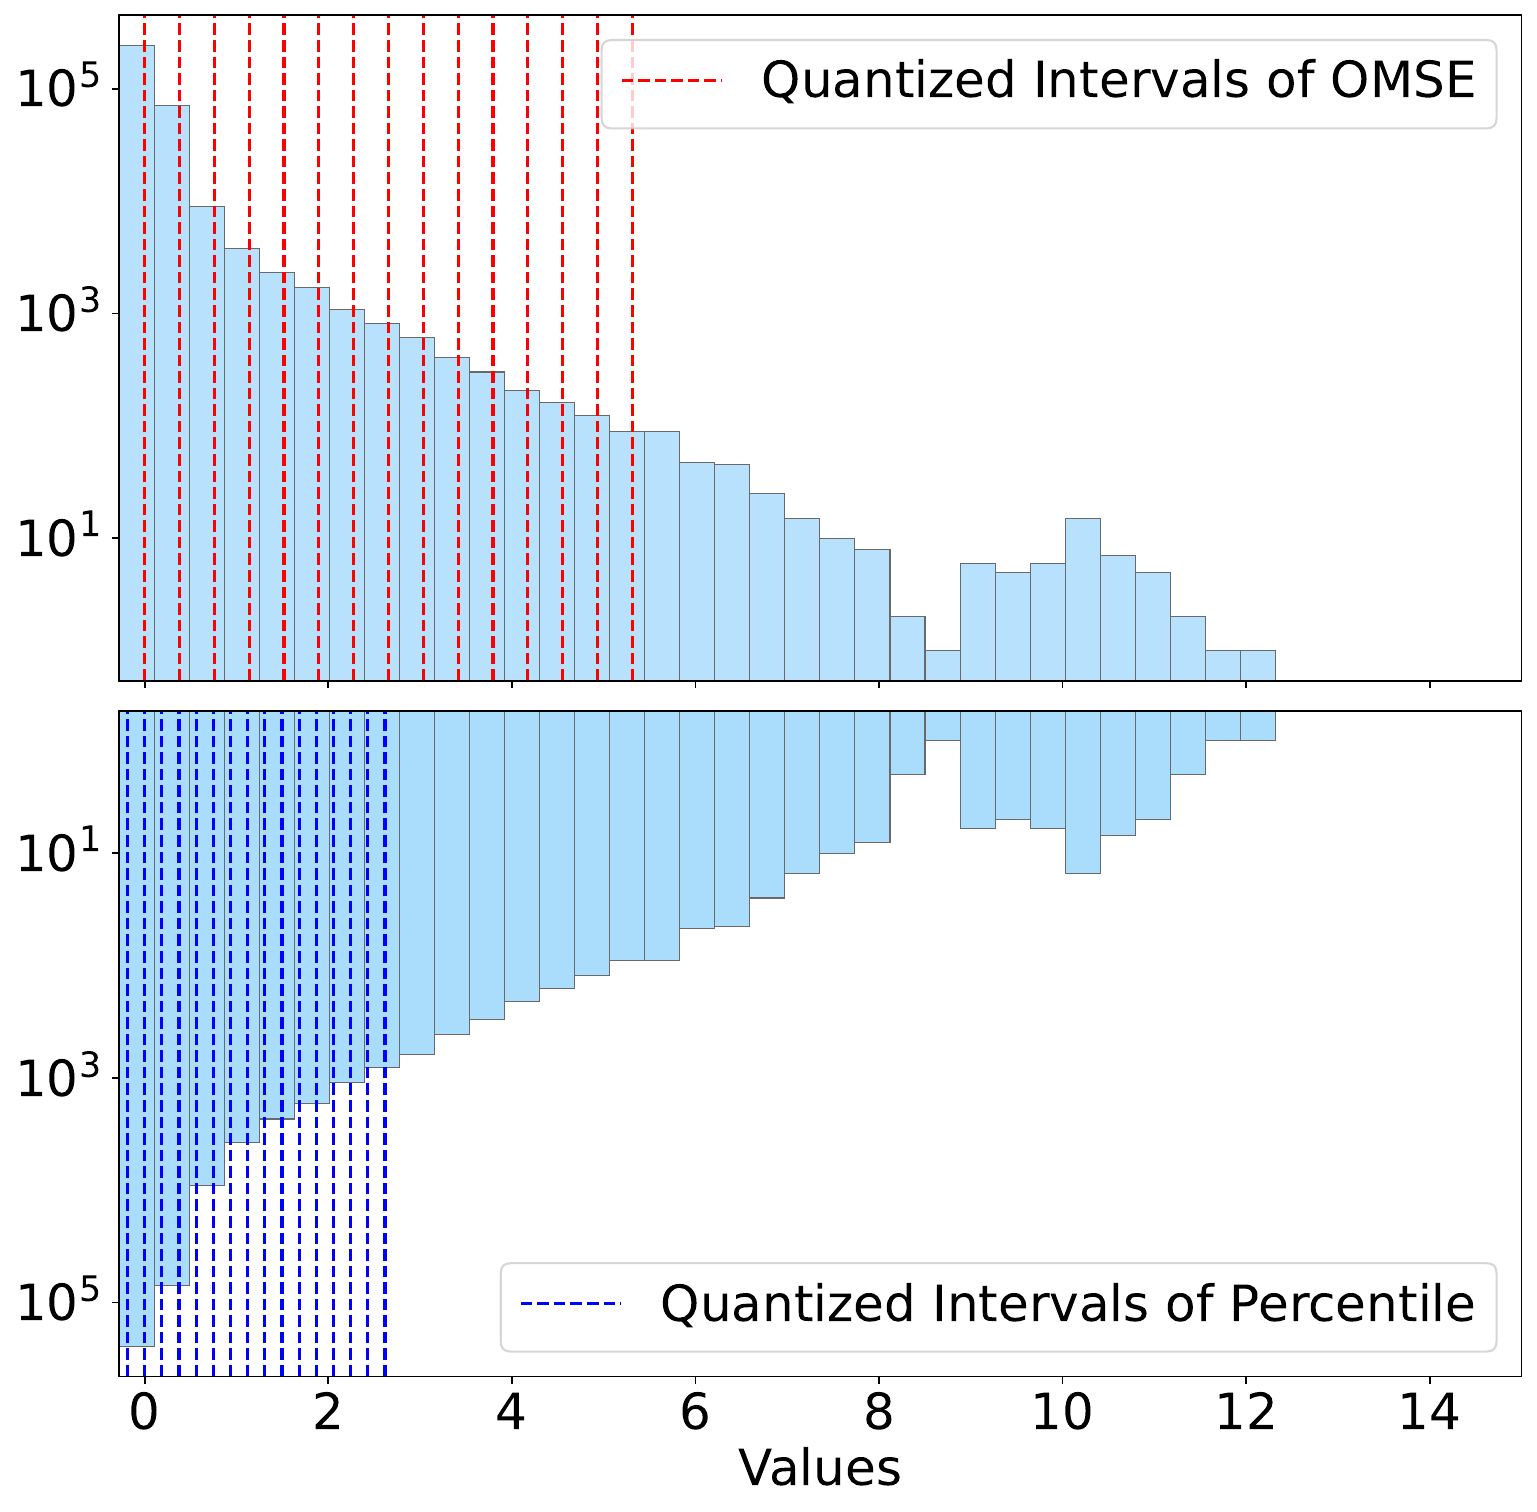}
  }
  % \vspace{-2.5mm}
  \caption{The statistics of inputs $x_t$, which are observed on SSMs (forward branch) of Vim-S using a batch of size 32 randomly sampled from ImageNet. (a) The red and blue points represent the upper bounds of the 4-bit quantization intervals obtained using OMSE or Percentile initialization, respectively. The horizontal axis presents observations across SSMs within different layers. (b) The 4-bit quantization intervals are initialized using OMSE or Percentile on the 5-th SSM of Vim-S, respectively.}
  \label{outlier}
  % \vspace{-4mm}
\end{figure}

In order to explain the reason why OMSE~\cite{OMSE} initialization is worse than Percentile~\cite{percentile} initialization in the low bit case, we take an example of 4-bit activation quantization on inputs $x_t$ using OMSE or Percentile, where $x_t$ are inputs of the state equation ($h_t=\overline{A}_th_{t-1}+\overline{B}_tx_t$). As shown in Fig.~\ref{outlier:box}, affected by large-scale outliers, the upper bounds of quantization intervals of OMSE are significantly larger than those of Percentile. As demonstrated in Fig.~\ref{outlier:hist}, large quantization intervals of OMSE in the low bit case lead to coarse-grained quantization with a large quantization error in densely distributed regions.
