# Supplementary material for: QMamba: Post-Training Quantization for Vision State Space Models
Source: arXiv:2501.13624 source file (2025-01-23)
Supplement: Supplementary file 2 [file qmamba_framework.tex]

\section{More Details of Quantized Mamba Block}
\label{qmamba_framework}

The implementation details of quantized Mamba block using our QMamba framwork is shown in Fig.~\ref{qmamba_framework}, which demonstrates quantization settings for linear projections and the causal convolution layer in a Mamba block excluding the SSM. Since the optional branch is not used in VMamba~\cite{vmamba}, we do not quantize the optional branch of Vim~\cite{vim} and keep it floating-point. 
For the bit settings in our experiments, we follow BRECQ~\cite{brecq} to set 8-bit weights and activations for the first and the last layer of Vim and VMamba.
In addition, as demonstrated in Fig.~\ref{qmamba_framework}, we also set 8-bit activations for some linear projections and causal convolutions to focus on the activation quantization in SSM. 

% \begin{figure}[t]
%   \centering
%   \includegraphics[width=0.83\linewidth]{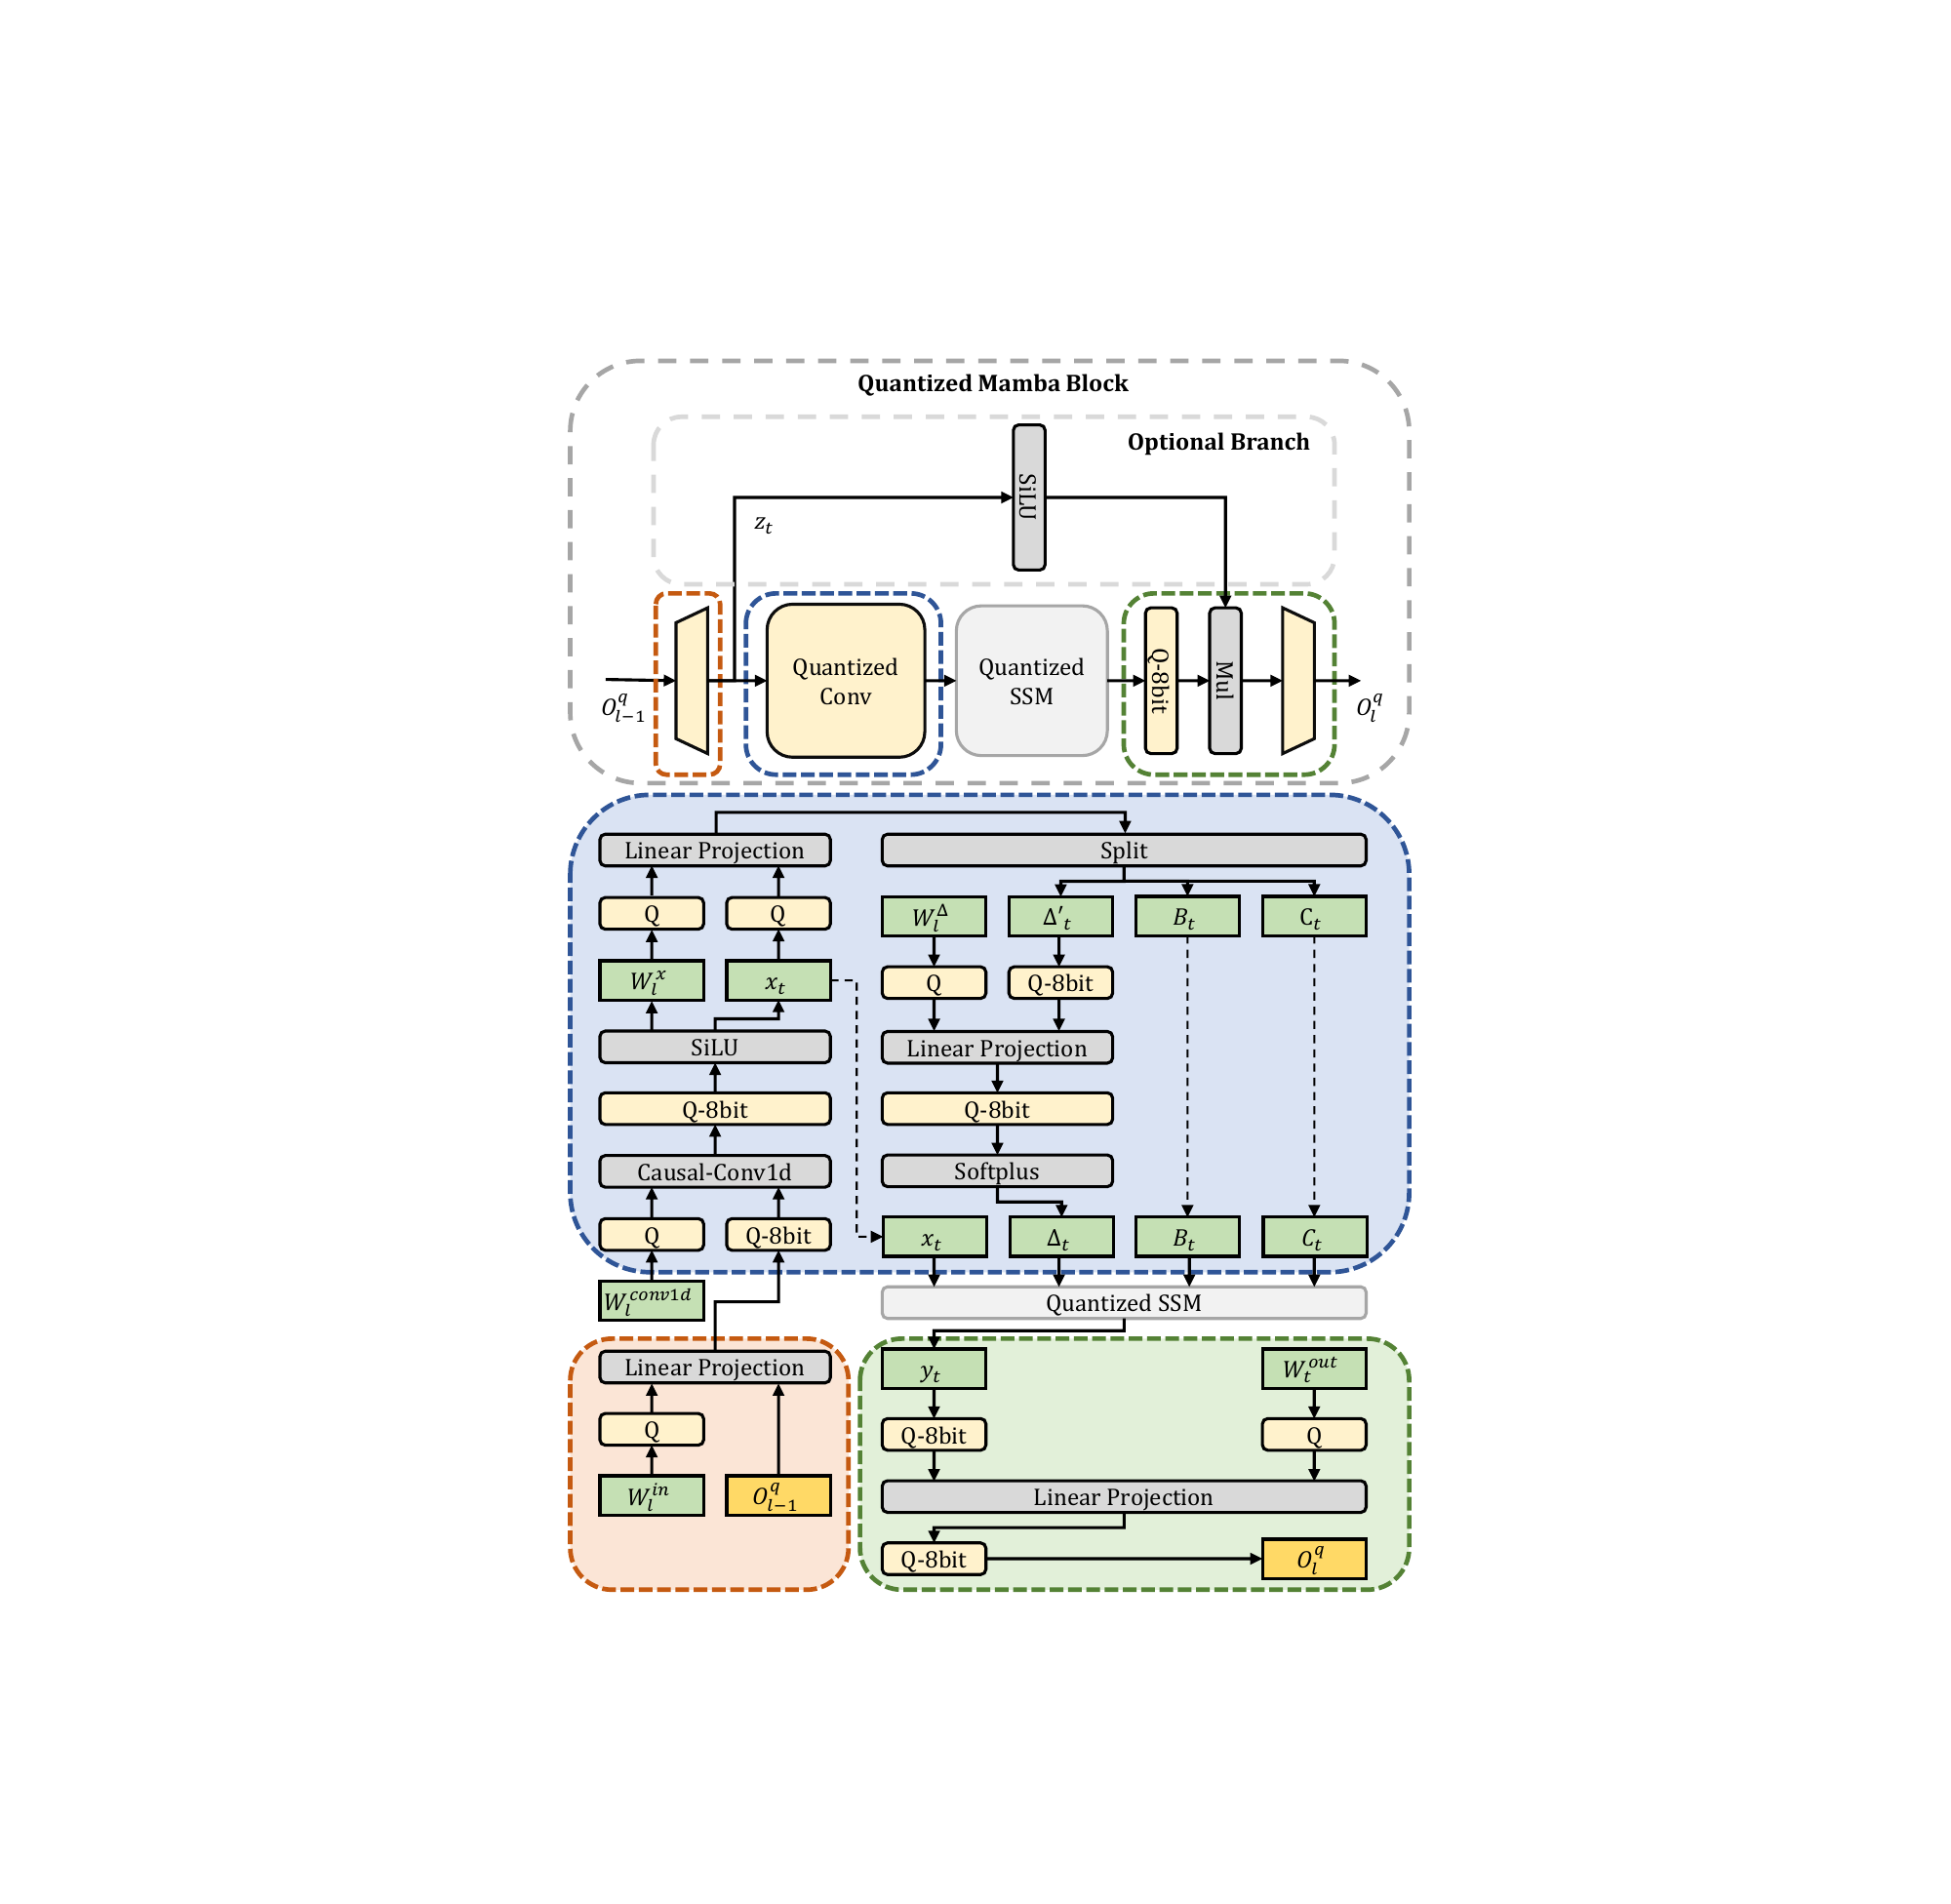}
%   \vspace{-1.5mm}
%   \caption{More details of quantized Mamba block using our QMamba framework. $W^{in}_l$, $W^{x}_l$, $W^{\Delta}_l$, and $W^{out}_l$ are weigths of linear projections in the $l$-th SSM. $W^{conv1d}_l$ represents the weight of the causal convolution. \textit{Q-8bit} means we use 8-bit tensor-wise uniform quantization. The optional branch is not quantized.}
%   \label{qmamba_framework}
%   \vspace{-4mm}
% \end{figure}

\begin{figure}[t]
  \centering
  \includegraphics[width=0.83\linewidth]{supp-pic/supp_main_pic2.pdf}
  % \vspace{-1.5mm}
  \caption{More details of quantized Mamba block using our QMamba framework. $W^{in}_l$, $W^{x}_l$, $W^{\Delta}_l$, and $W^{out}_l$ are weigths of linear projections in the $l$-th SSM. $W^{conv1d}_l$ represents the weight of the causal convolution. \textit{Q-8bit} means we use 8-bit tensor-wise uniform quantization. The optional branch is not quantized.}
  \label{qmamba_framework}
  % \vspace{-4mm}
\end{figure}
