# Supplementary material for: QMamba: Post-Training Quantization for Vision State Space Models
Source: arXiv:2501.13624 source file (2025-01-23)
Supplement: Supplementary file 5 [file median.tex]

\section{Analysis on the Skewness Condition}
\label{median}

% \begin{figure}[tp]
%   \centering
%   \subcaptionbox{\label{abl:scale_change1}}{
%     \includegraphics[width=0.485\linewidth]{supp-pic/scale_change/vim_b_box_16.pdf}%0.342
%   }\hfill %\hspace{0.01\textwidth}
%   \subcaptionbox{\label{abl:scale_change2}}{
%     \includegraphics[width=0.48\linewidth]{supp-pic/scale_change/vim_b_hist_16.pdf}
%   }
%   % \vspace{-2.5mm}
%   \caption{The visualization of our TGQ on hidden states at different time steps in Vim. (a) The variation of hidden states $h_t$ and TGQ scaling factors with time steps. The horizontal axis represents the time step. (b) The distribution of hidden states  at different time step and the corresponding quantized values using our TGQ. }
%   \label{abl:TGQ}
%   % \vspace{-4mm}
% \end{figure}

\begin{figure*}[t]
  \centering
  \subcaptionbox{Vim-T\label{median:vim:t}}{
    \begin{minipage}{0.32\linewidth}
      \centering
      \includegraphics[width=\linewidth]{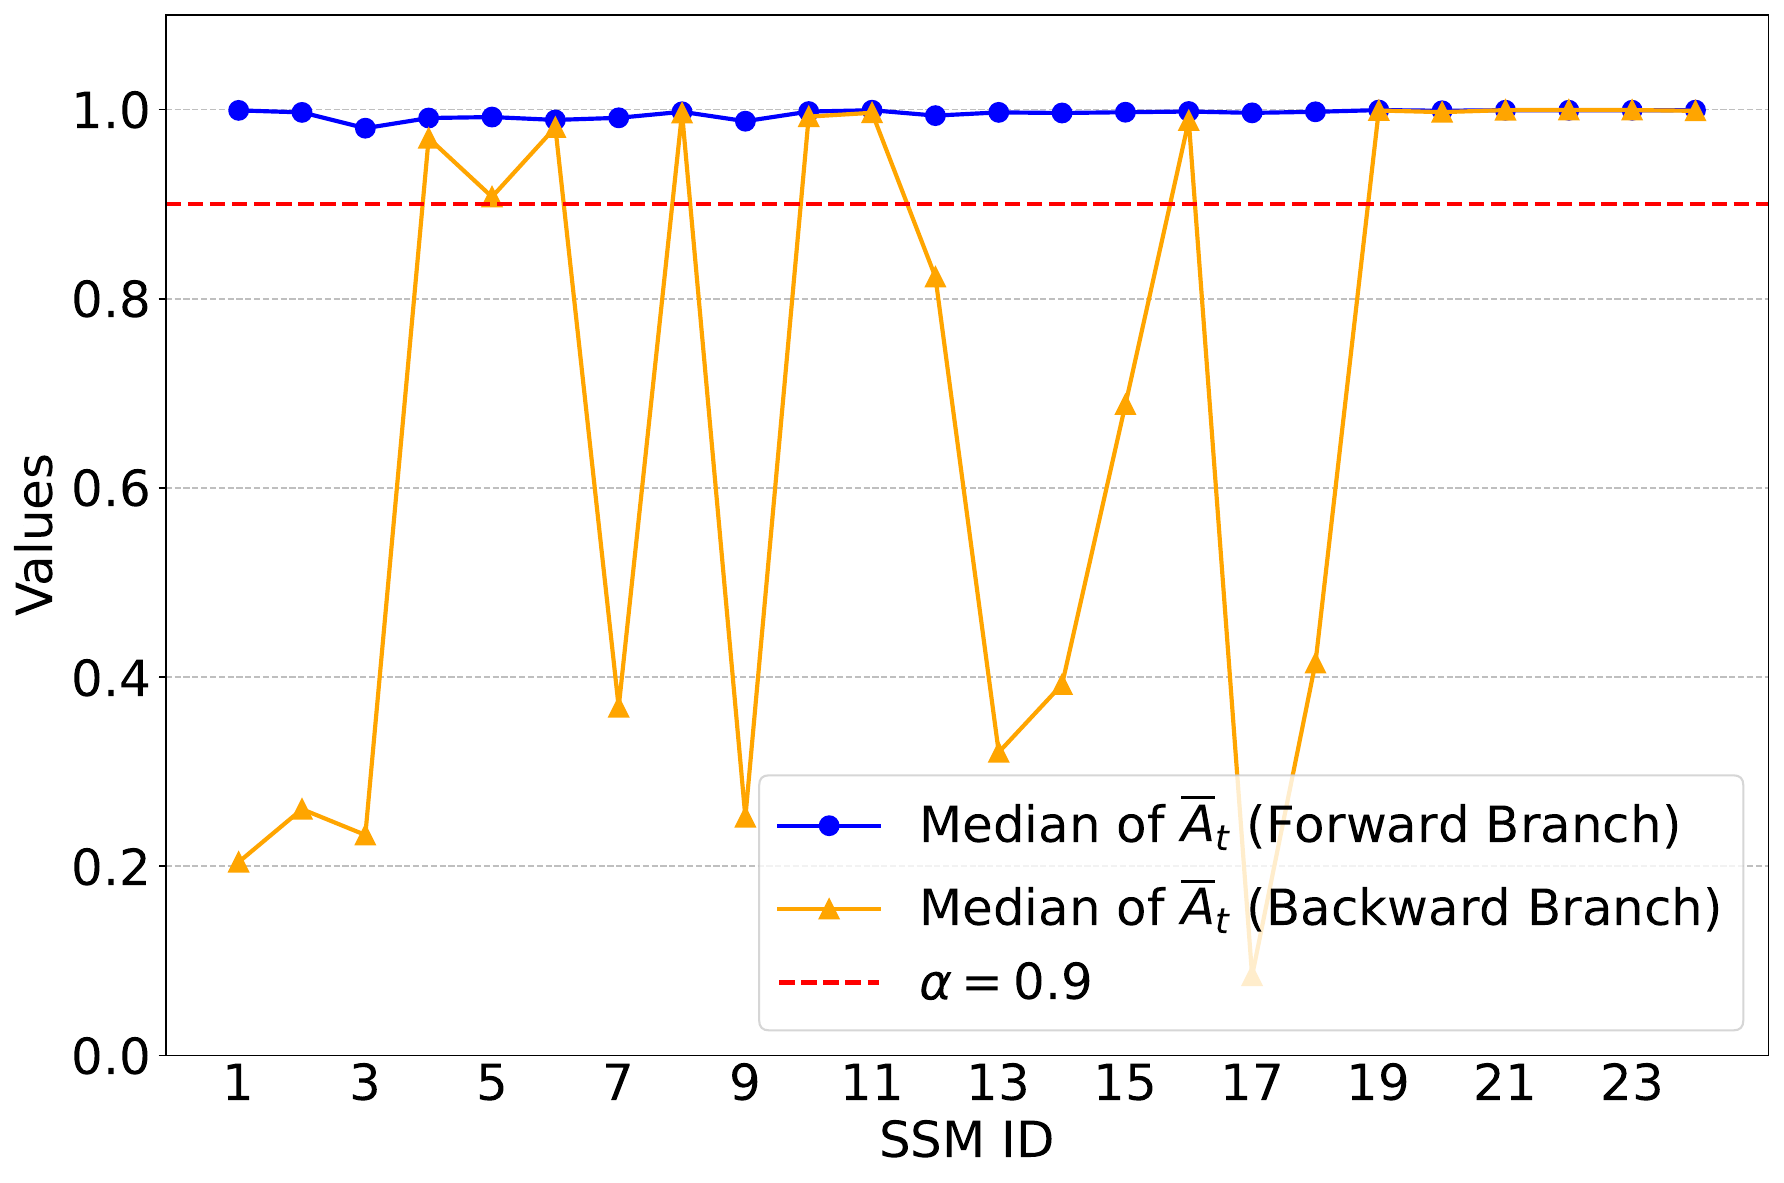}
    \end{minipage}
  }\hfill %\hspace{0.01\textwidth}
  \subcaptionbox{Vim-S\label{median:vim:s}}{
    \begin{minipage}{0.32\linewidth}
      \centering
      \includegraphics[width=\linewidth]{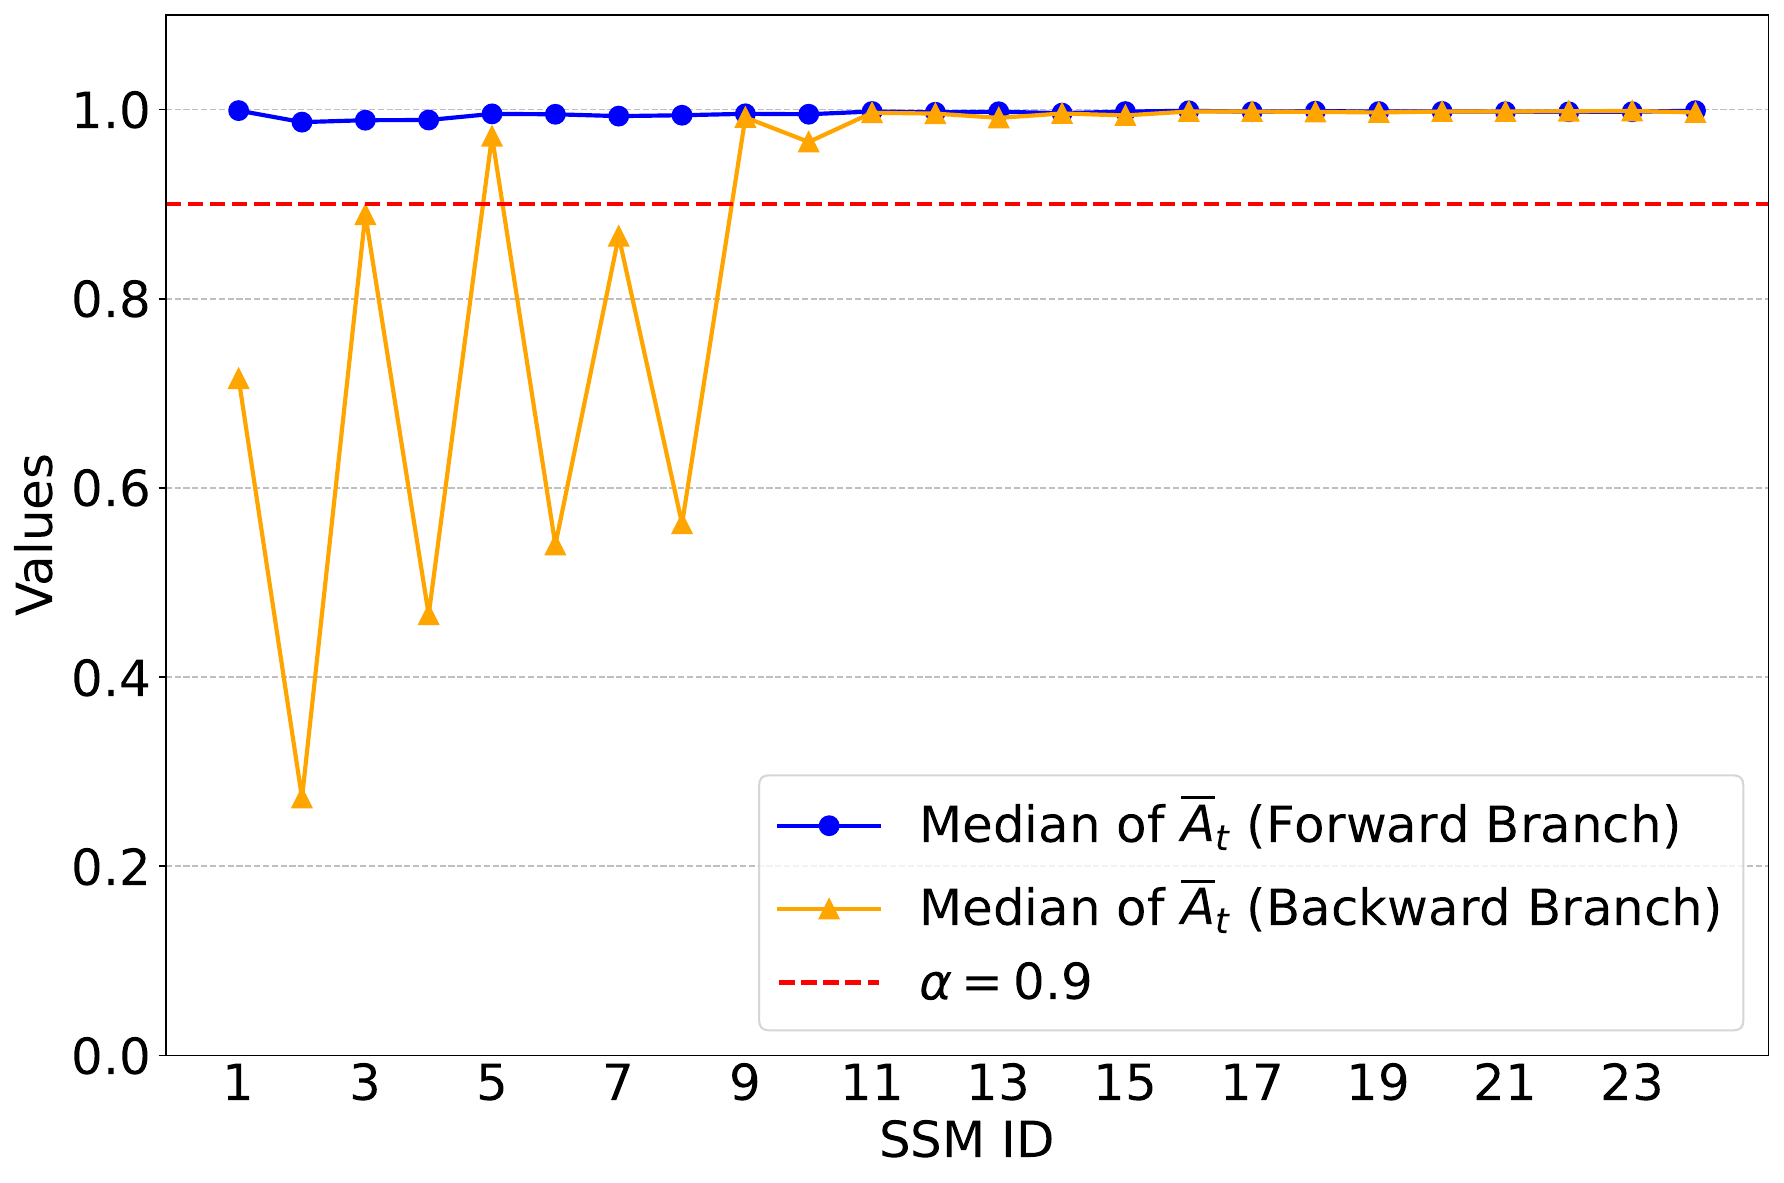}
    \end{minipage}
  }\hfill %\hspace{0.01\textwidth}
  \subcaptionbox{Vim-B\label{median:vim:b}}{
    \begin{minipage}{0.32\linewidth}
      \centering
      \includegraphics[width=\linewidth]{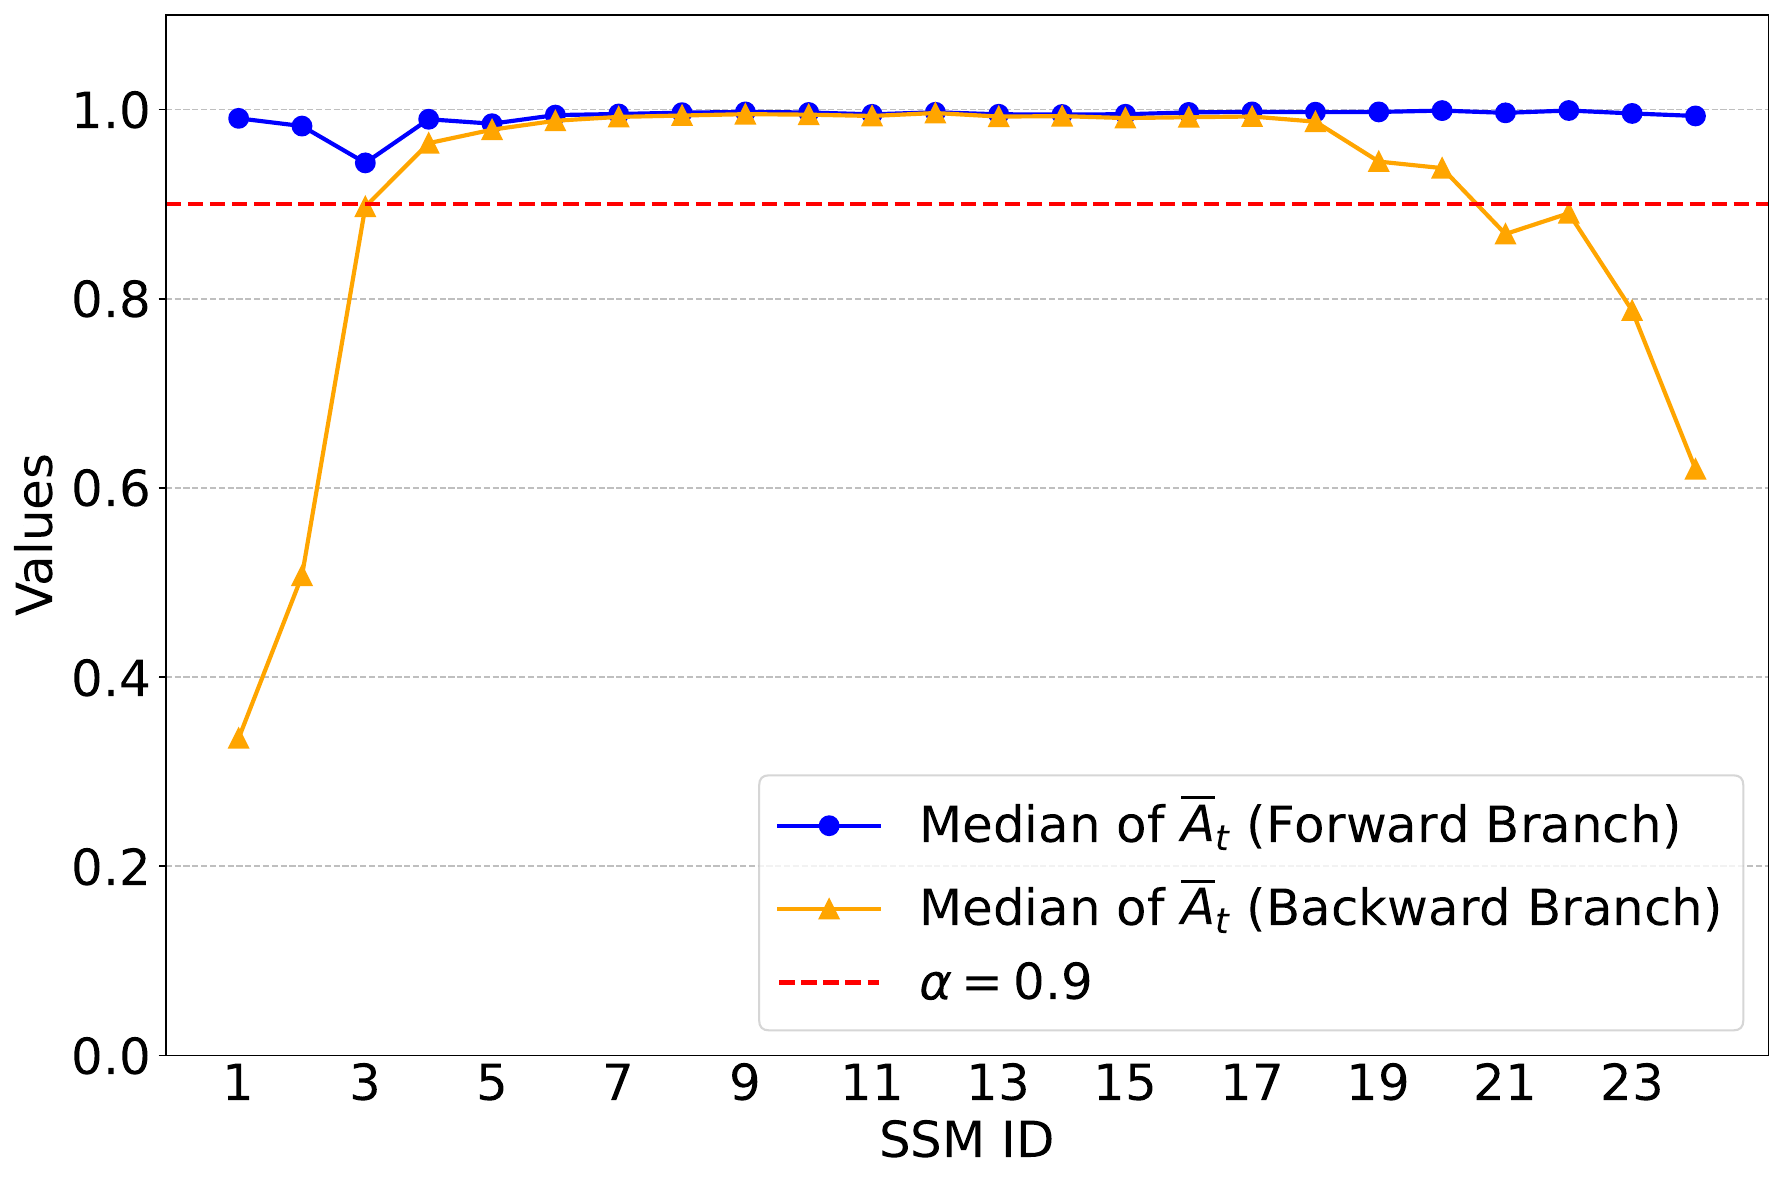}
    \end{minipage}
  } \\

  \subcaptionbox{VMamba-T\label{median:vmamba:t}}{
    \begin{minipage}{0.32\linewidth}
      \centering
      \includegraphics[width=\linewidth]{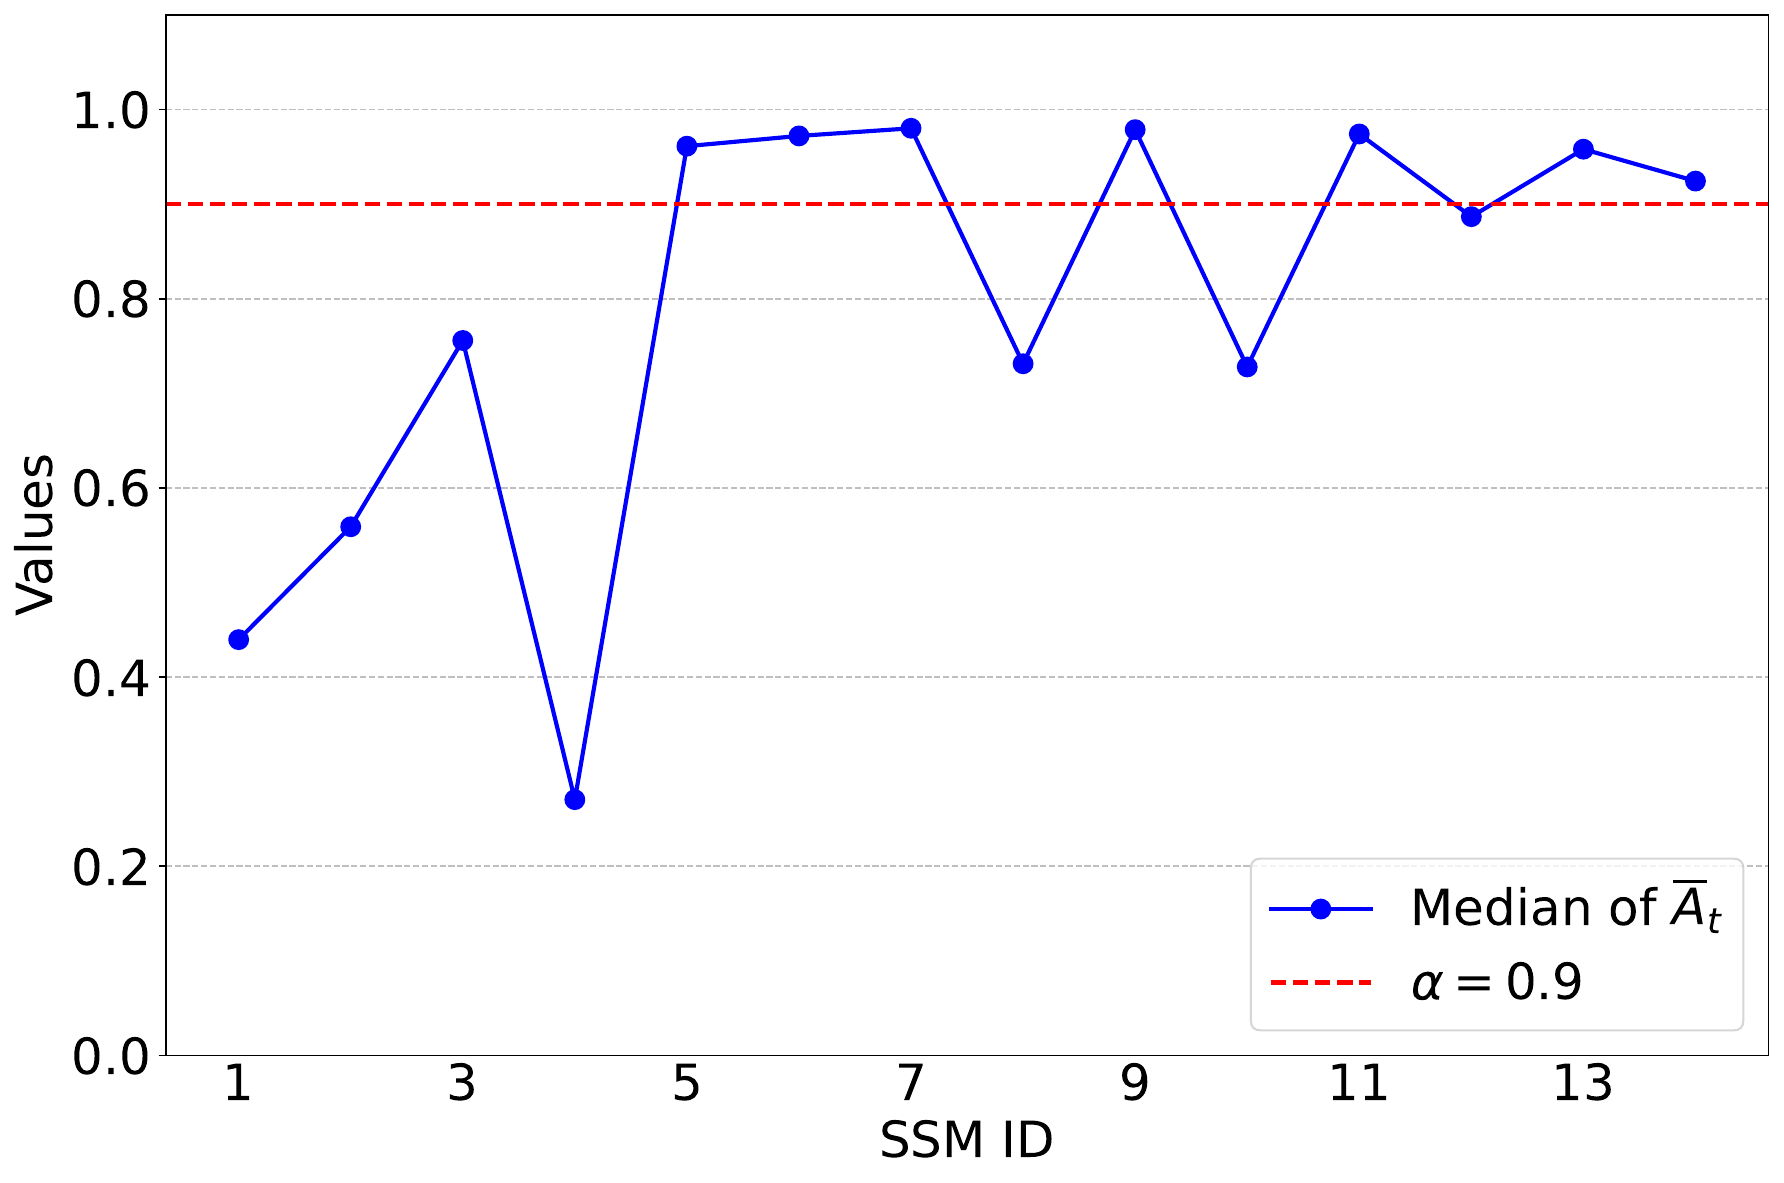}
    \end{minipage}
  }\hfill %\hspace{0.01\textwidth}
  \subcaptionbox{VMamba-S\label{median:vmamba:s}}{
    \begin{minipage}{0.32\linewidth}
      \centering
      \includegraphics[width=\linewidth]{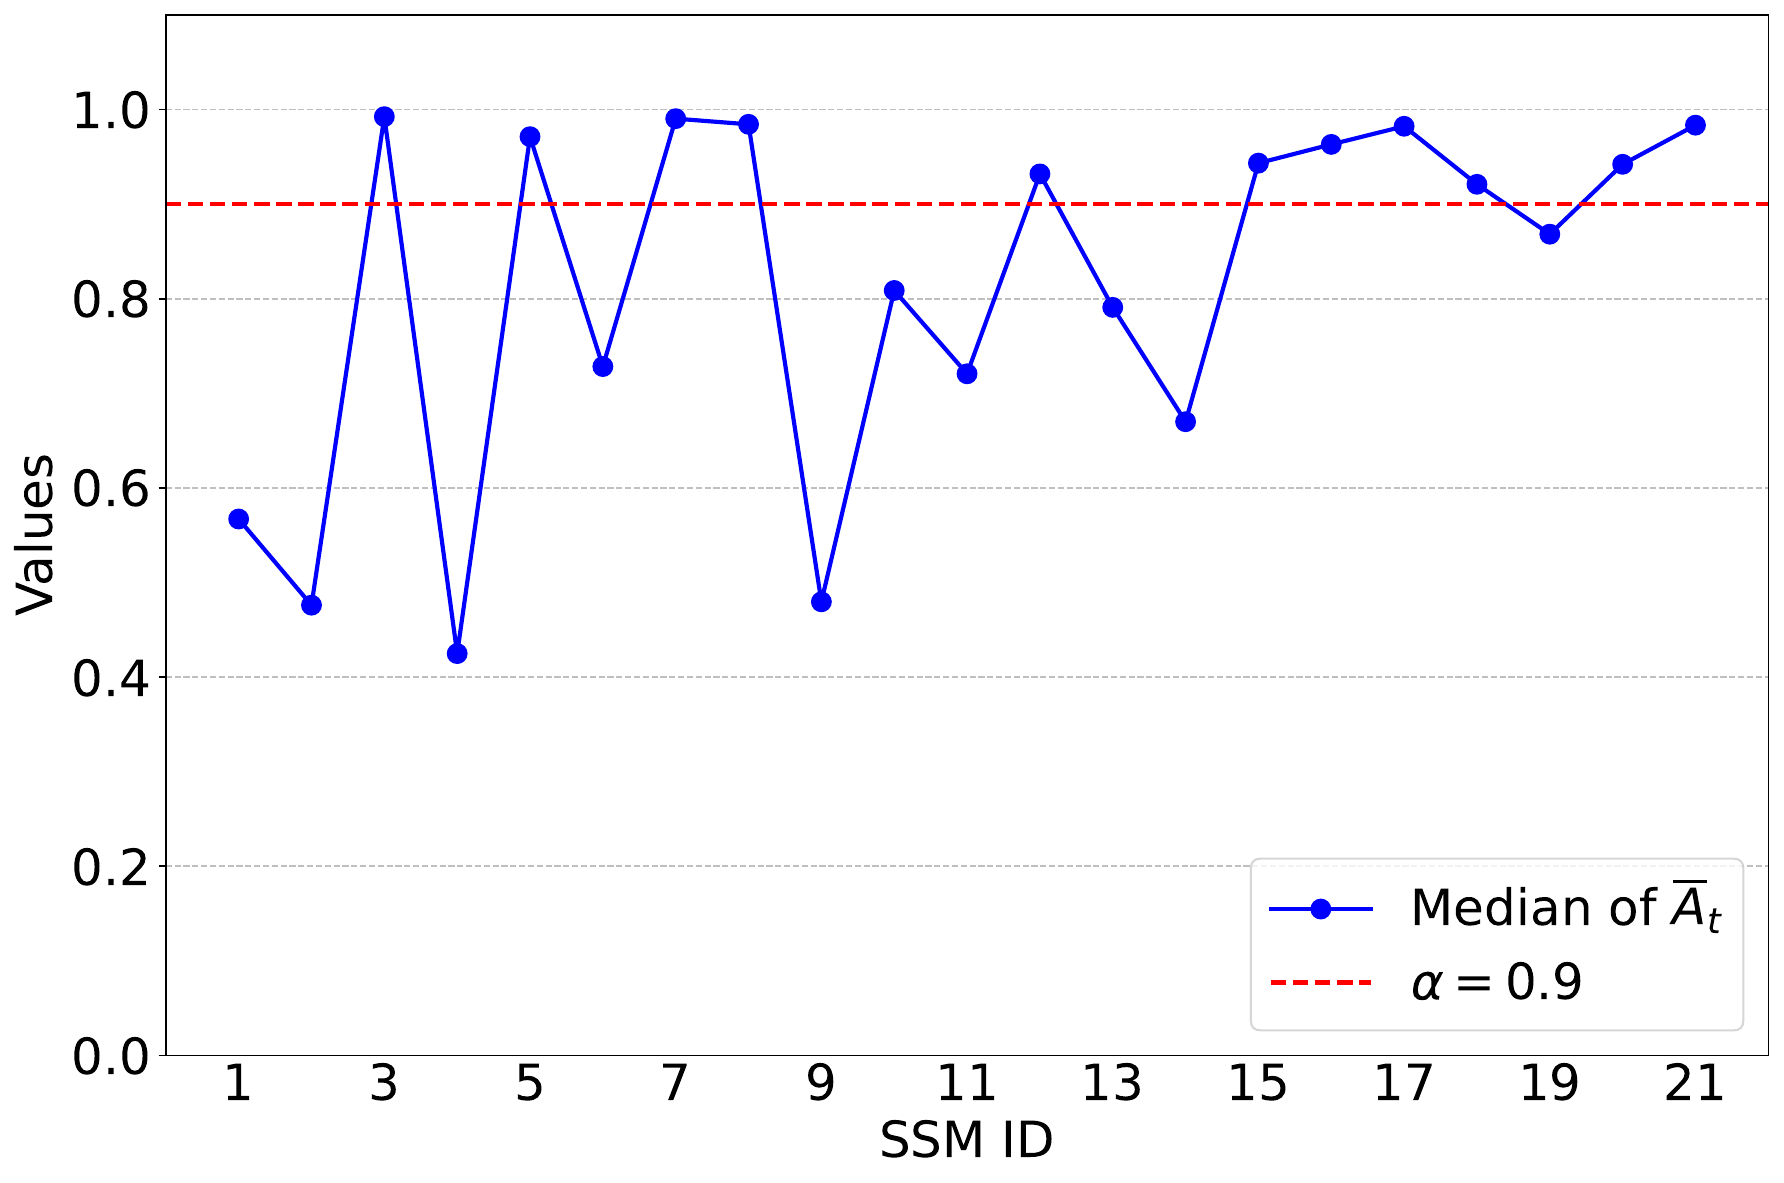}
    \end{minipage}
  }\hfill %\hspace{0.01\textwidth}
  \subcaptionbox{VMamba-B\label{median:vmamba:b}}{
    \begin{minipage}{0.32\linewidth}
      \centering
      \includegraphics[width=\linewidth]{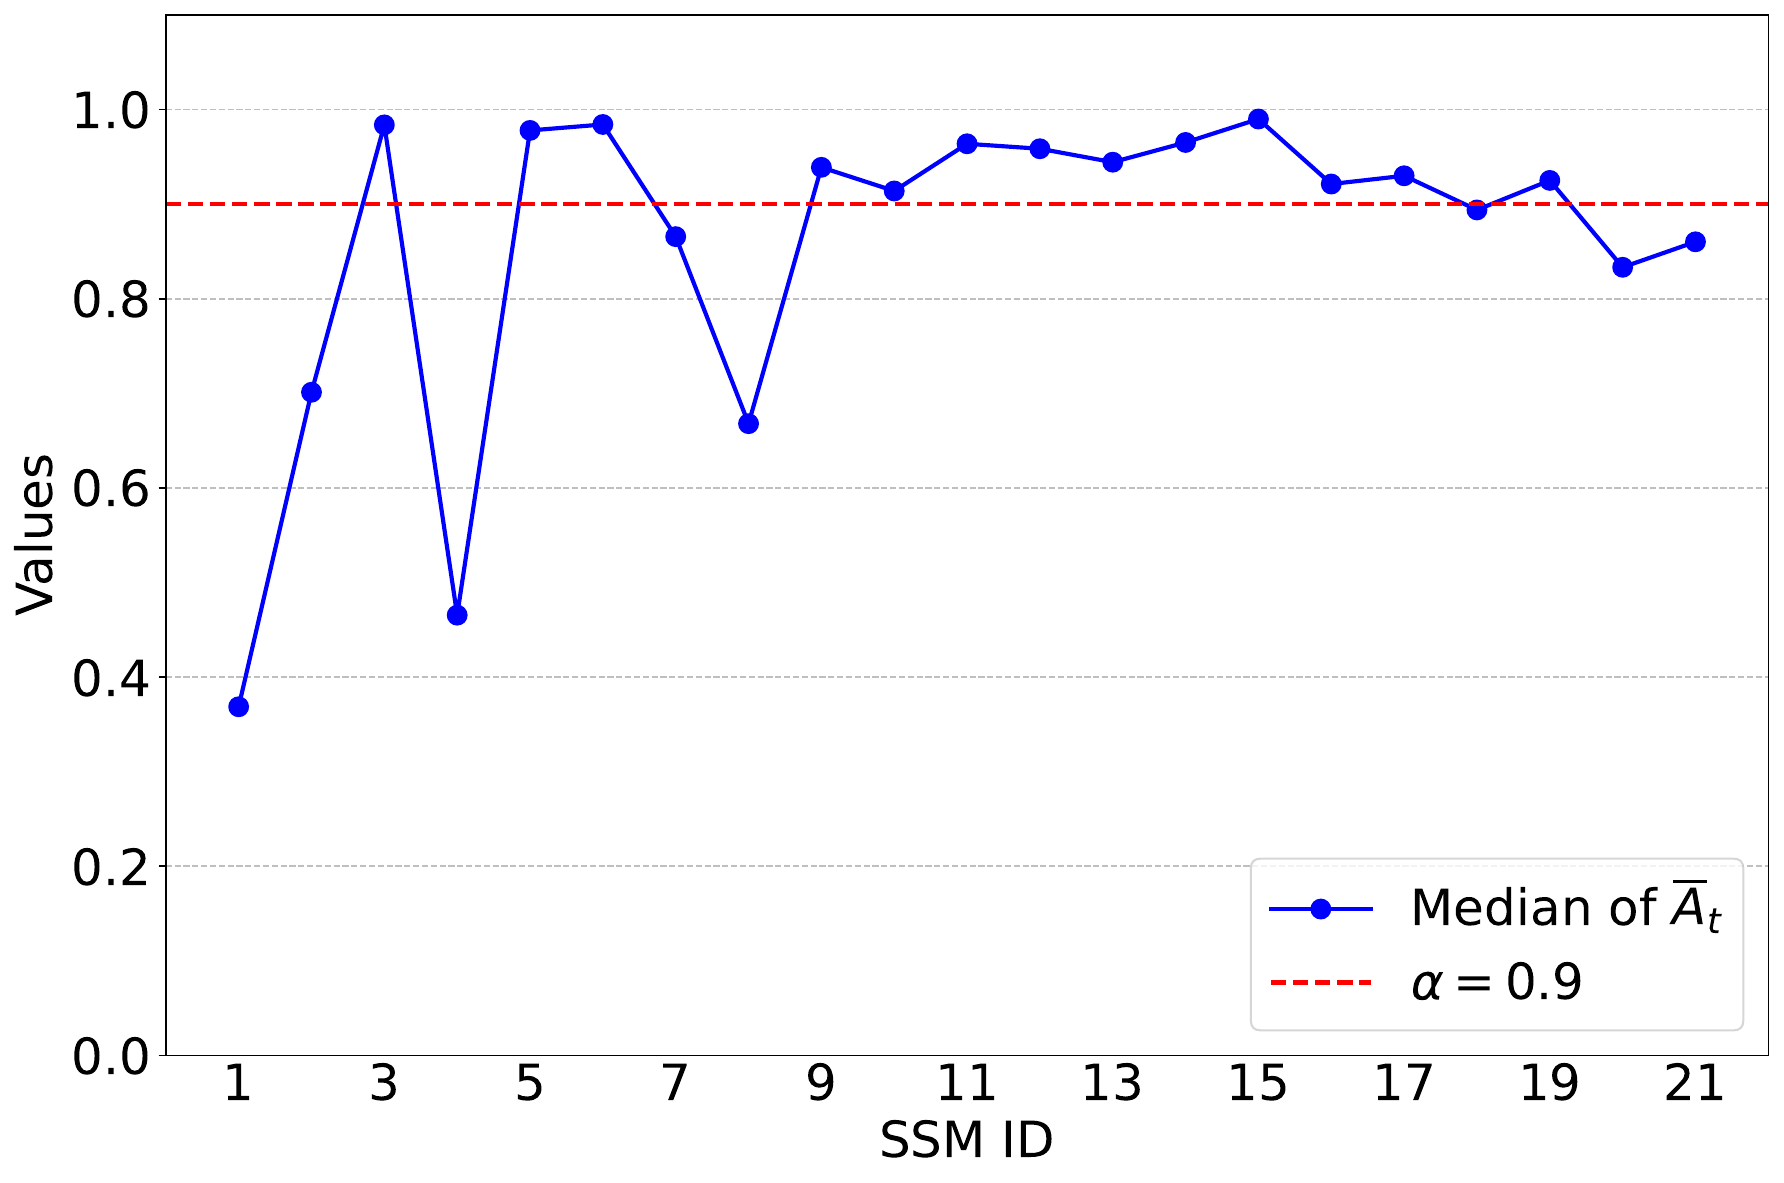}
    \end{minipage}
  }
  \vspace{-3mm}
  \caption{The median values of discrete parameters $\overline{A}_t$ in each SSM of Vim~\cite{vim} and VMamba~\cite{vmamba}, which are calculated using a batch of size 32 randomly sampled from ImageNet. $\alpha$ is the skewness boundary and set to 0.9 as default. The horizontal axis (SSM ID) presents observations across SSMs within different layers. The forward branch and the backward branch constitute bidirectional SSMs in Vim.}
  \label{median:ssm}
\end{figure*}

As mentioned in our paper, our proposed LtSQ determines whether the distribution of discrete parameters $\overline{A}_t$ exhibits long-tailed skewness based on median values, \emph{i.e.}, the skewness condition: $Median_{1\leq t \leq L}(\overline{A}_t)>\alpha$. 
SSMs whose median values of $\overline{A}_t$ are greater than the skewness boundary $\alpha$ will use LtSQ to quantize $\overline{A}_t$, otherwise, they will use uniform quantization. Here, we calculate median values of $\overline{A}_t$ in each SSM of Vim and VMamba. As shown in Fig.~\ref{median}, the median values of $\overline{A}_t$ in most SSMs of Vim and VMamba are greater than $\alpha$, indicating that these SSMs use LtSQ to quantize discrete parameters $\overline{A}_t$.
