# Supplementary material for: QMamba: Post-Training Quantization for Vision State Space Models
Source: arXiv:2501.13624 source file (2025-01-23)
Supplement: Supplementary file 6 [file observation.tex]

\section{More Visualizations of the Distribution}
\label{observation}

We visualize distributions of discrete parameters $\overline{A}_t$ and hidden states $h_t$ in SSMs of multiple versions of Vim~\cite{vim} and VMamba~\cite{vmamba}, which are observed on a batch of size 4 randomly sampled from ImageNet. As mentioned in our paper, the visualizations provided show highly dynamic changes of $h_t$ and long-tailed skewness of $\overline{A}_t$. Specifically, in these examples, the highly dynamic changes of hidden states include 1) gradual increases (Fig.~\ref{observation:vim:t:state_box}, Fig.~\ref{observation:vim:s:state_box}, Fig.~\ref{observation:vim:b:state_box}, and Fig.~\ref{observation:vmamba:t:state_box}), 2) periodic changes (Fig.~\ref{observation:vmamba:s:state_box}), and 3) increases followed by decreases (Fig.~\ref{observation:vmamba:b:state_box}).
