# Supplementary material for: QMamba: Post-Training Quantization for Vision State Space Models
Source: arXiv:2501.13624 source file (2025-01-23)
Supplement: Supplementary file 7 [file pic_ob_vim_base.tex]

\begin{figure*}[t]
  \centering
  \subcaptionbox{Distribution variations of $\overline{A}_t$\label{observation:vim:b:deltaA_box}}{
    \begin{minipage}{0.235\linewidth}
      \centering
      \includegraphics[width=\linewidth]{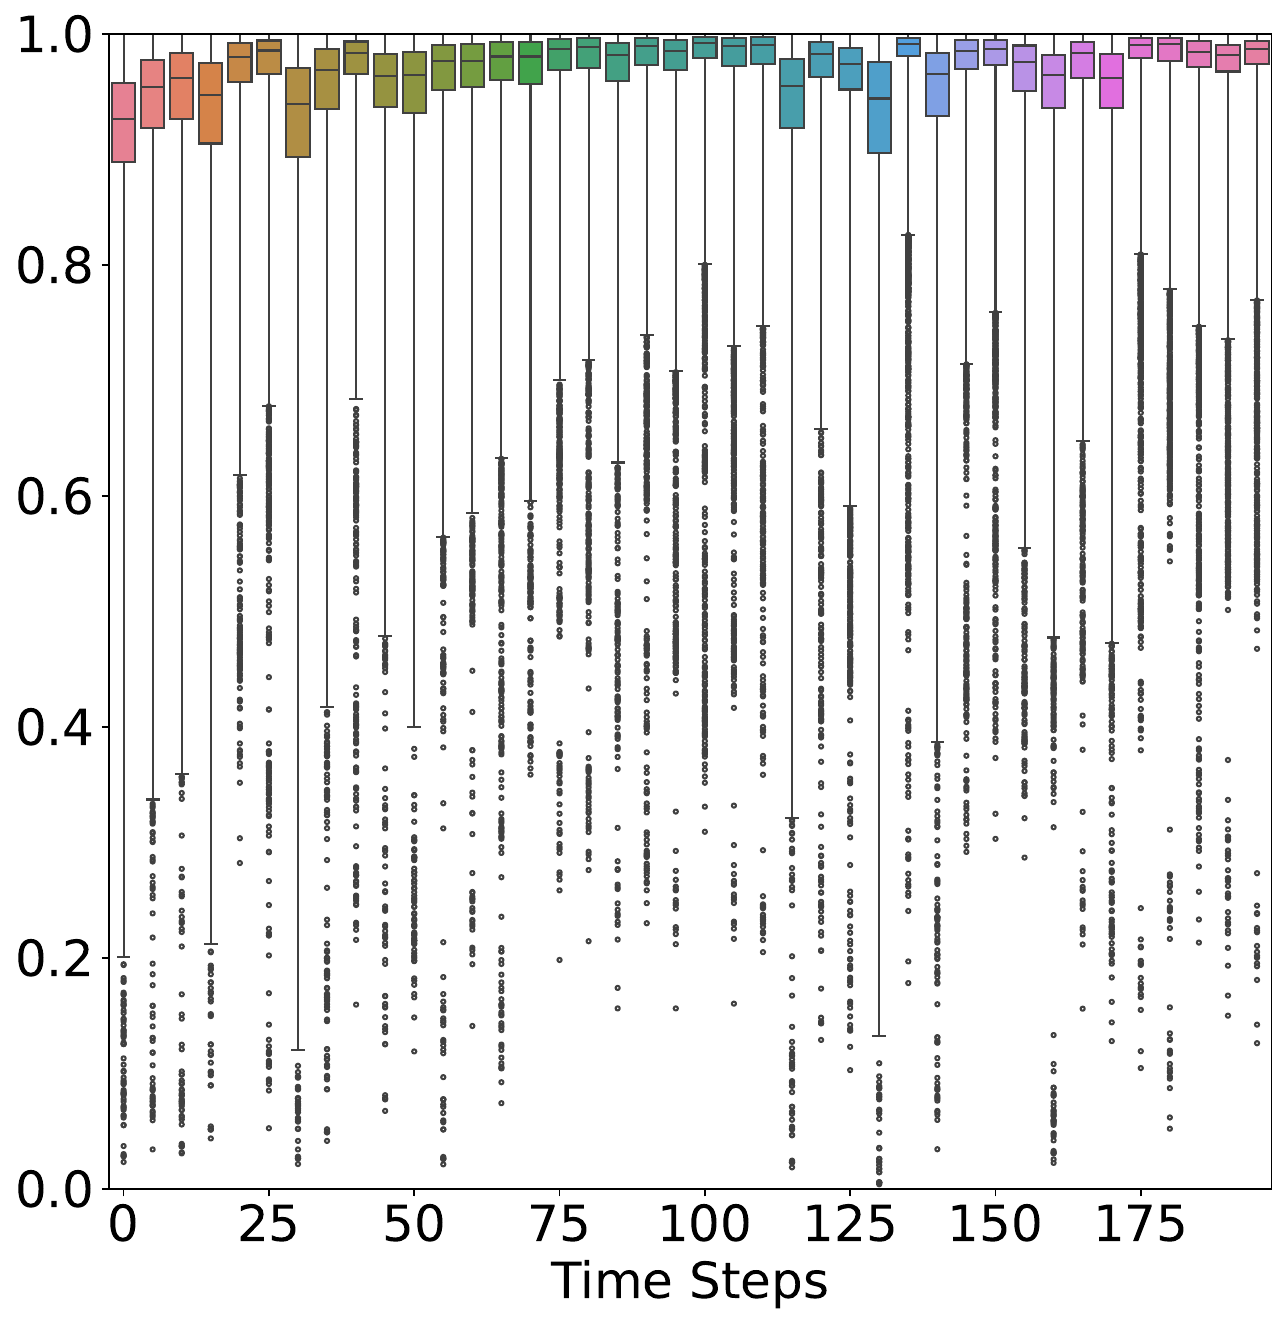}
    \end{minipage}
  }\hfill %\hspace{0.01\textwidth}
  \subcaptionbox{Distribution variations of $h_t$\label{observation:vim:b:state_box}}{
    \begin{minipage}{0.25\linewidth}
      \centering
      \includegraphics[width=\linewidth]{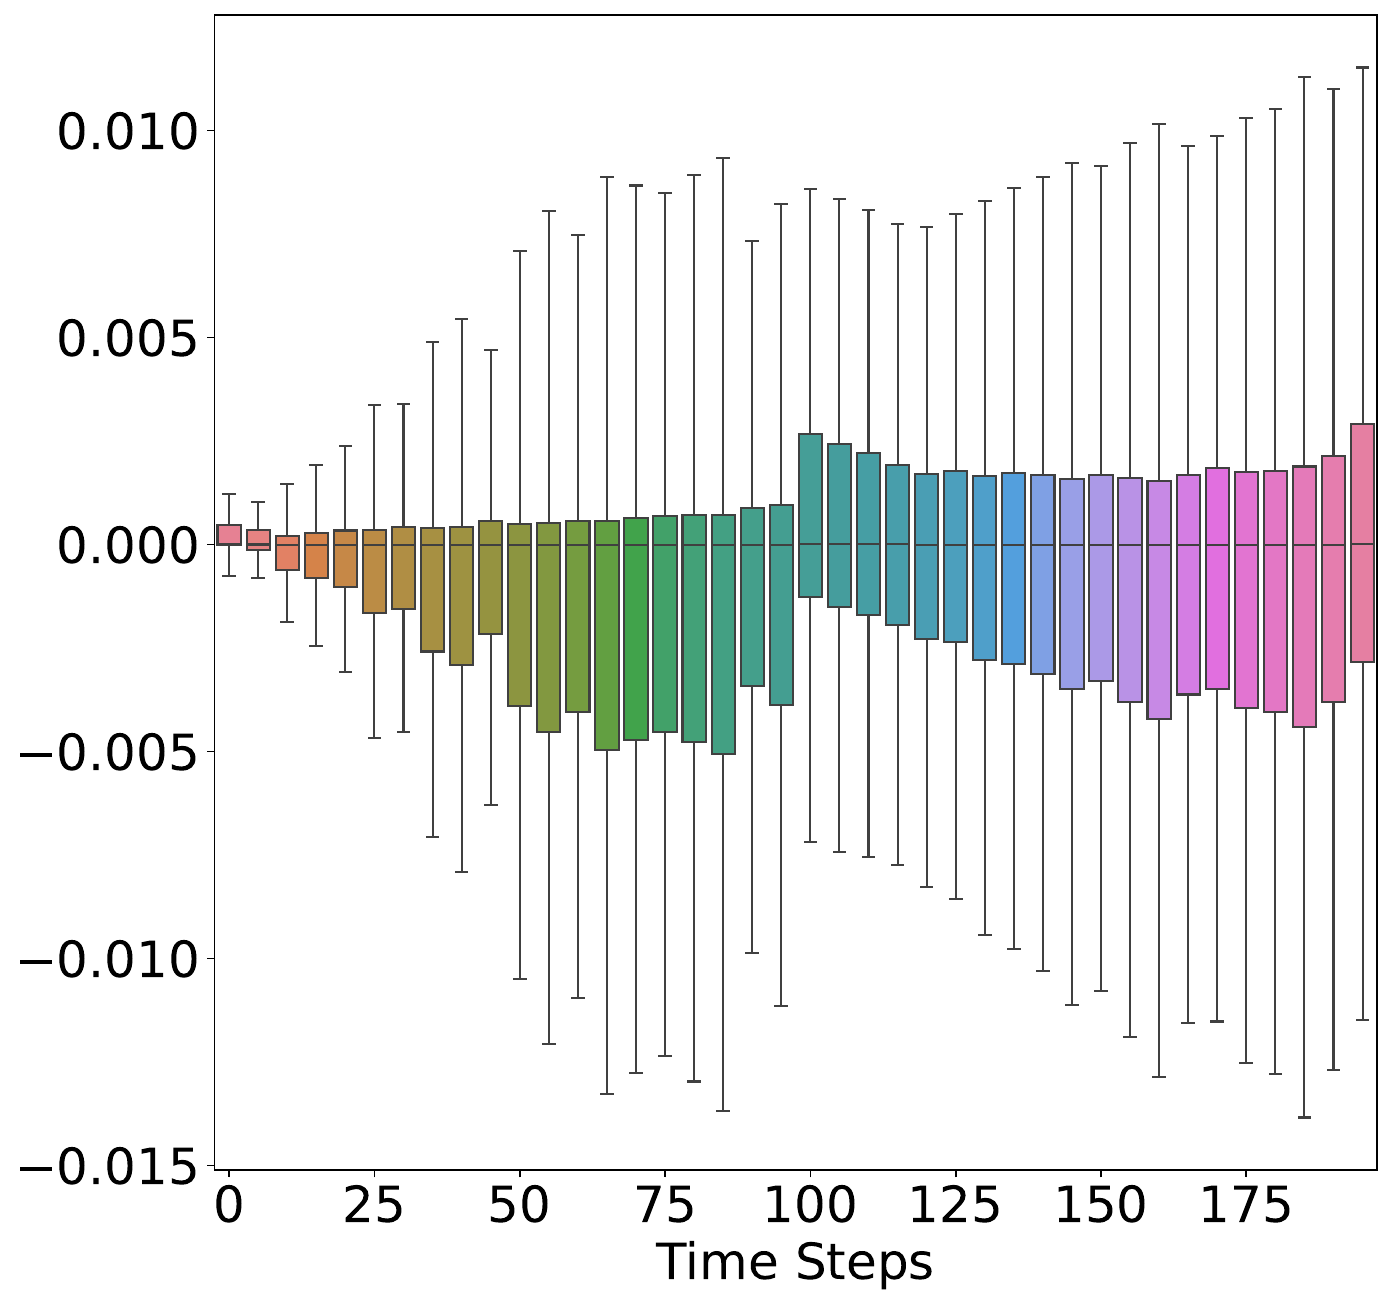}
    \end{minipage}
  }\hfill %\hspace{0.01\textwidth}
  \subcaptionbox{Uniform quantization on $\overline{A}_t$\label{observation:vim:b:deltaA_hist}}{
    \begin{minipage}{0.238\linewidth}
      \centering
      \includegraphics[width=\linewidth]{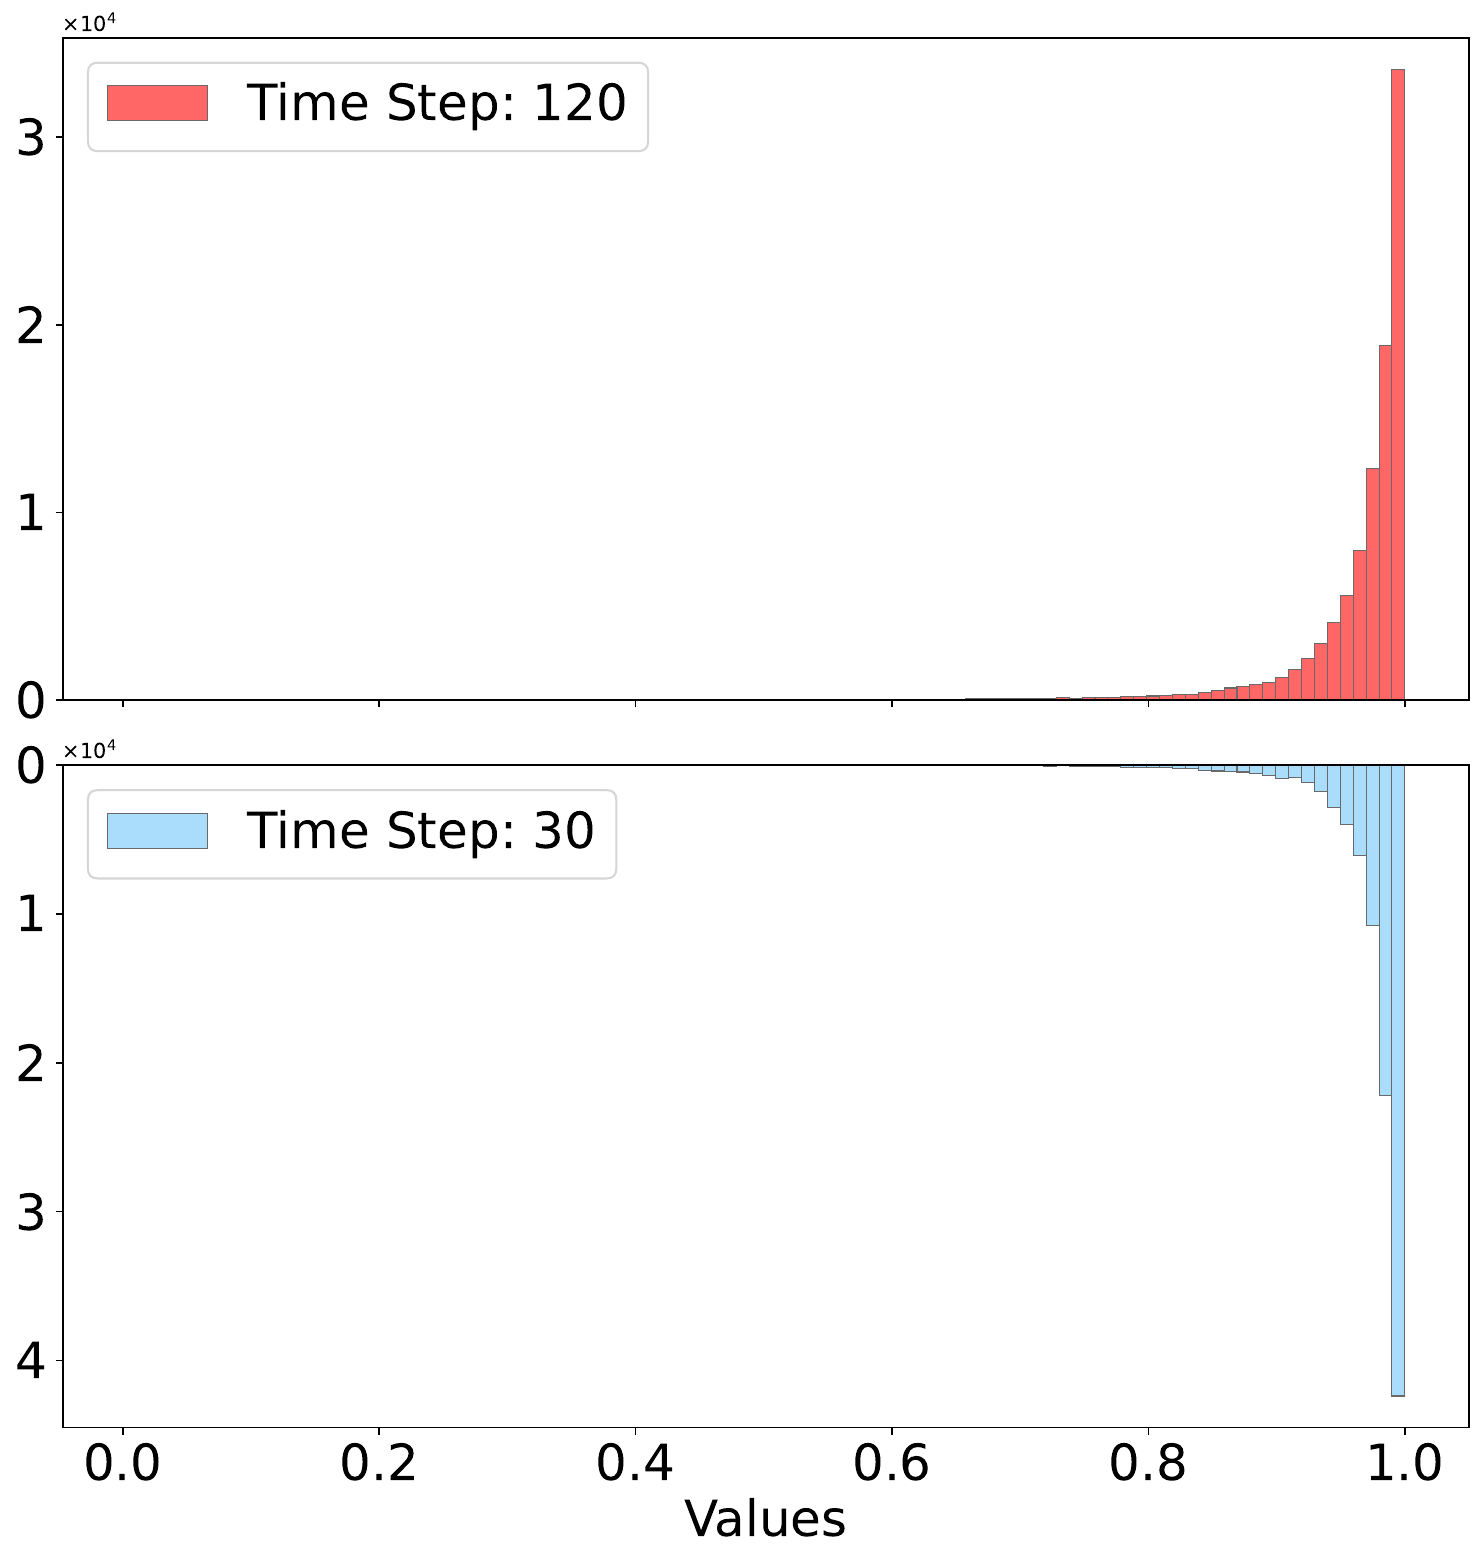}
    \end{minipage}
  }\hfill %\hspace{0.01\textwidth}
  \subcaptionbox{Uniform quantization on $h_t$\label{observation:vim:b:state_hist}}{
    \begin{minipage}{0.235\linewidth}
      \centering
      \includegraphics[width=\linewidth]{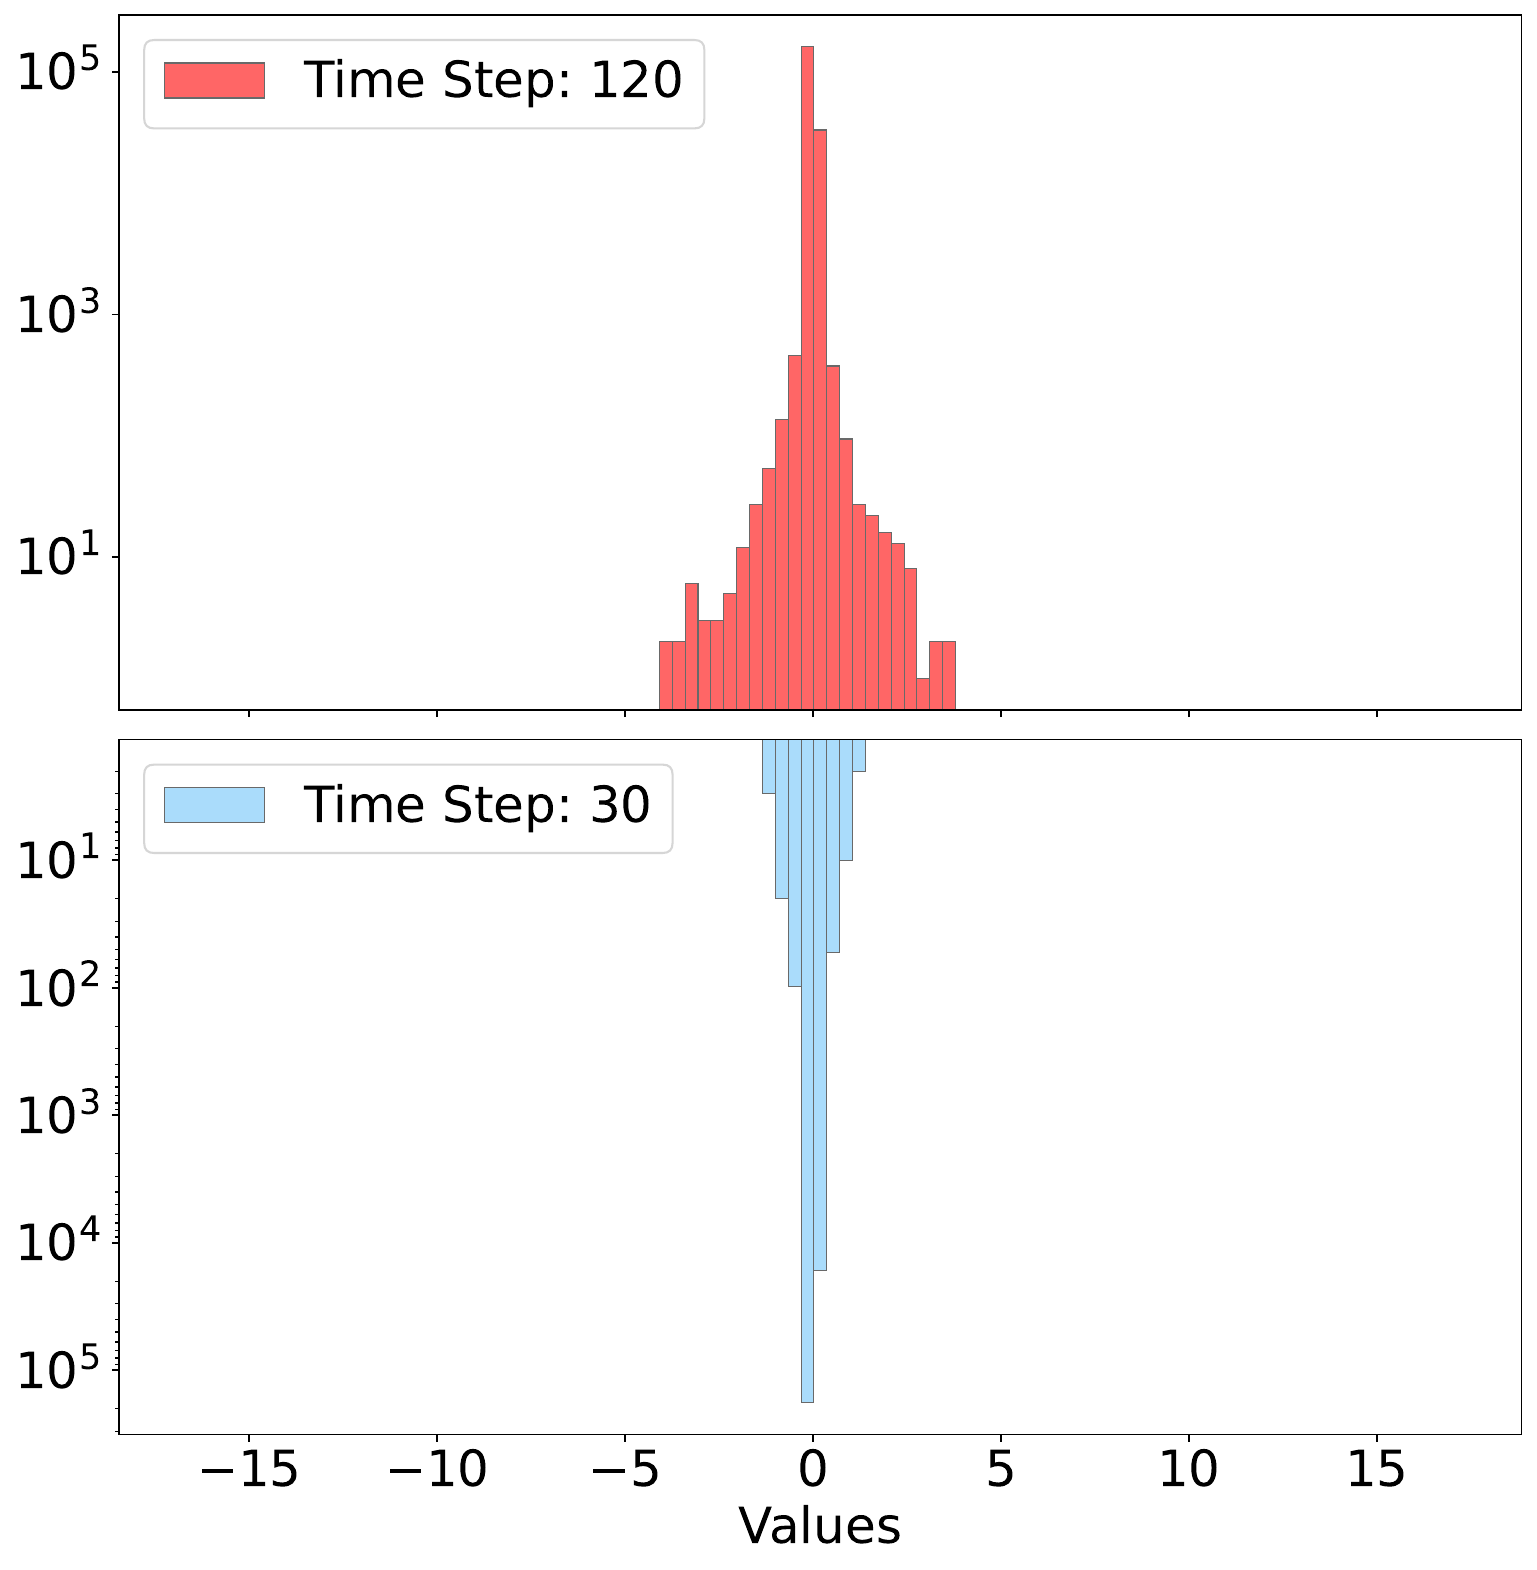}
    \end{minipage}
  }
  \caption{The statistics of discrete parameters $\overline{A}_t$ (5-th SSM) and hidden states $h_t$ (17-th SSM) are observed in the SSM of Vim-B~\cite{vim}. We visualize $\overline{A}_t$ and $h_t$ at every fifth time step in the sequence, and the outliers in the boxplot of $h_t$ are omitted for better visualization. The horizontal axis of (a) and (b) presents observations across different time steps.}
  \label{observation:vim:b}
\end{figure*}
