# Supplementary material for: QMamba: Post-Training Quantization for Vision State Space Models
Source: arXiv:2501.13624 source file (2025-01-23)
Supplement: Supplementary file 11 [file pic_ob_vmamba_small.tex]

\begin{figure*}[t]
  \centering
  \subcaptionbox{Distribution variations of $\overline{A}_t$\label{observation:vmamba:s:deltaA_box}}{
    \begin{minipage}{0.235\linewidth}
      \centering
      \includegraphics[width=\linewidth]{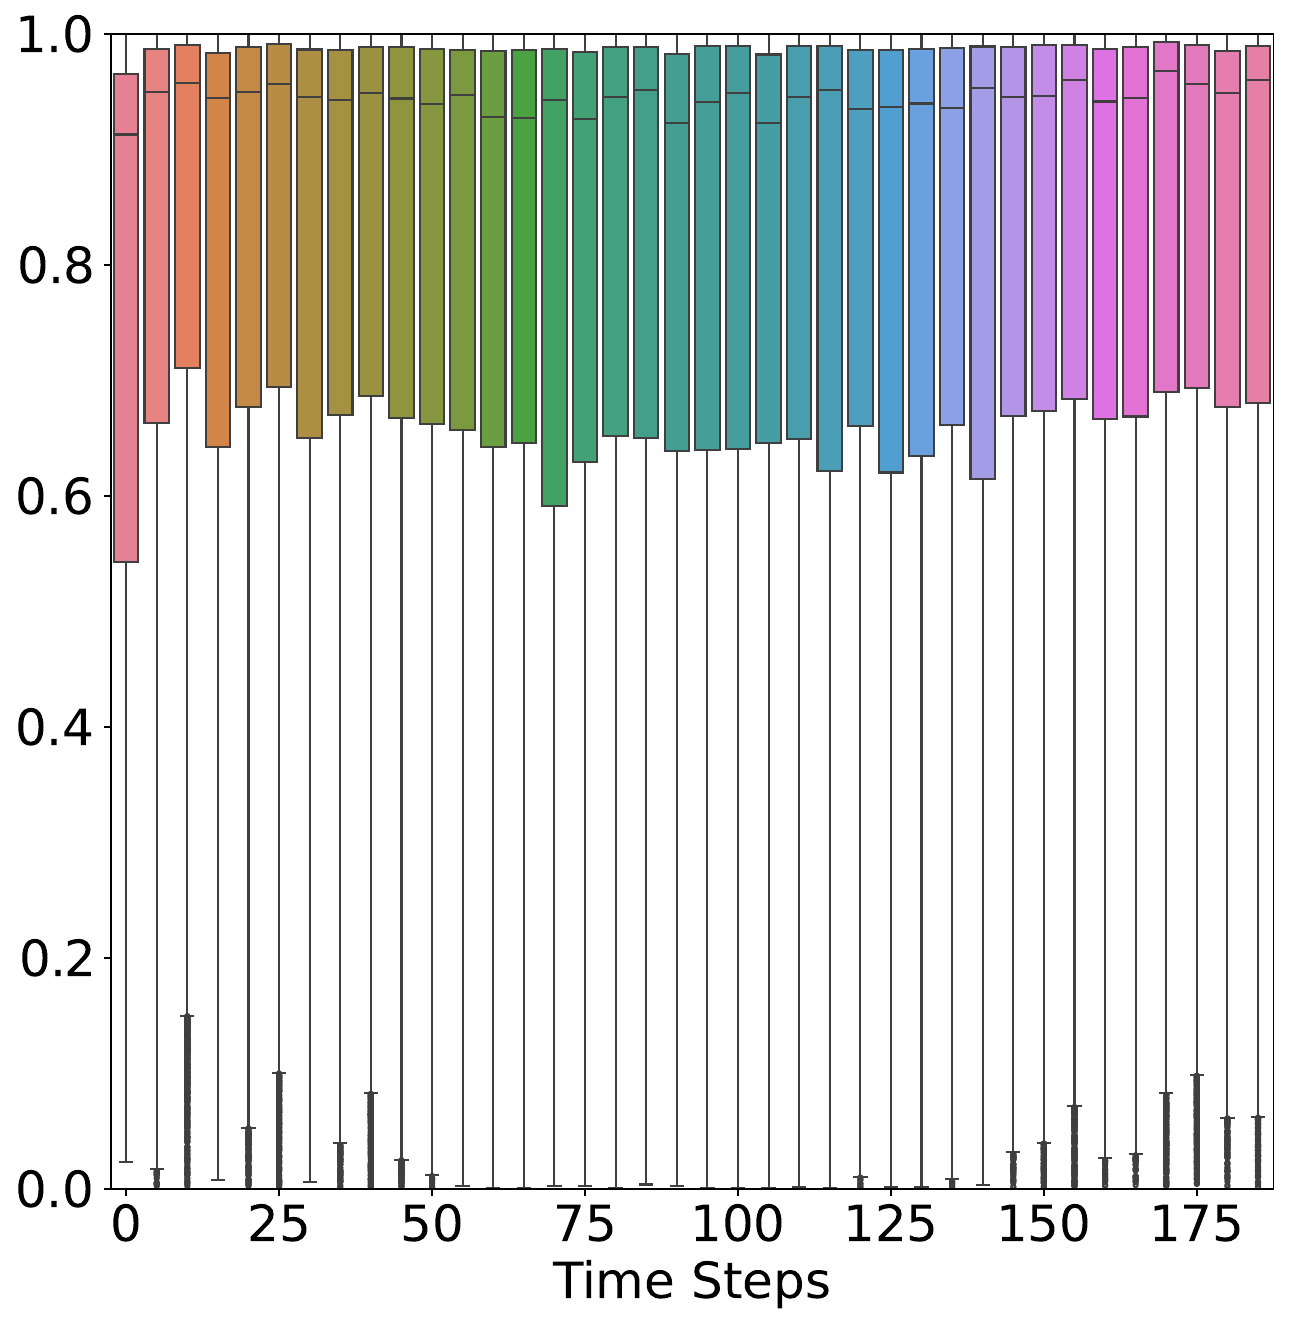}
    \end{minipage}
  }\hfill %\hspace{0.01\textwidth}
  \subcaptionbox{Distribution variations of $h_t$\label{observation:vmamba:s:state_box}}{
    \begin{minipage}{0.235\linewidth}
      \centering
      \includegraphics[width=\linewidth]{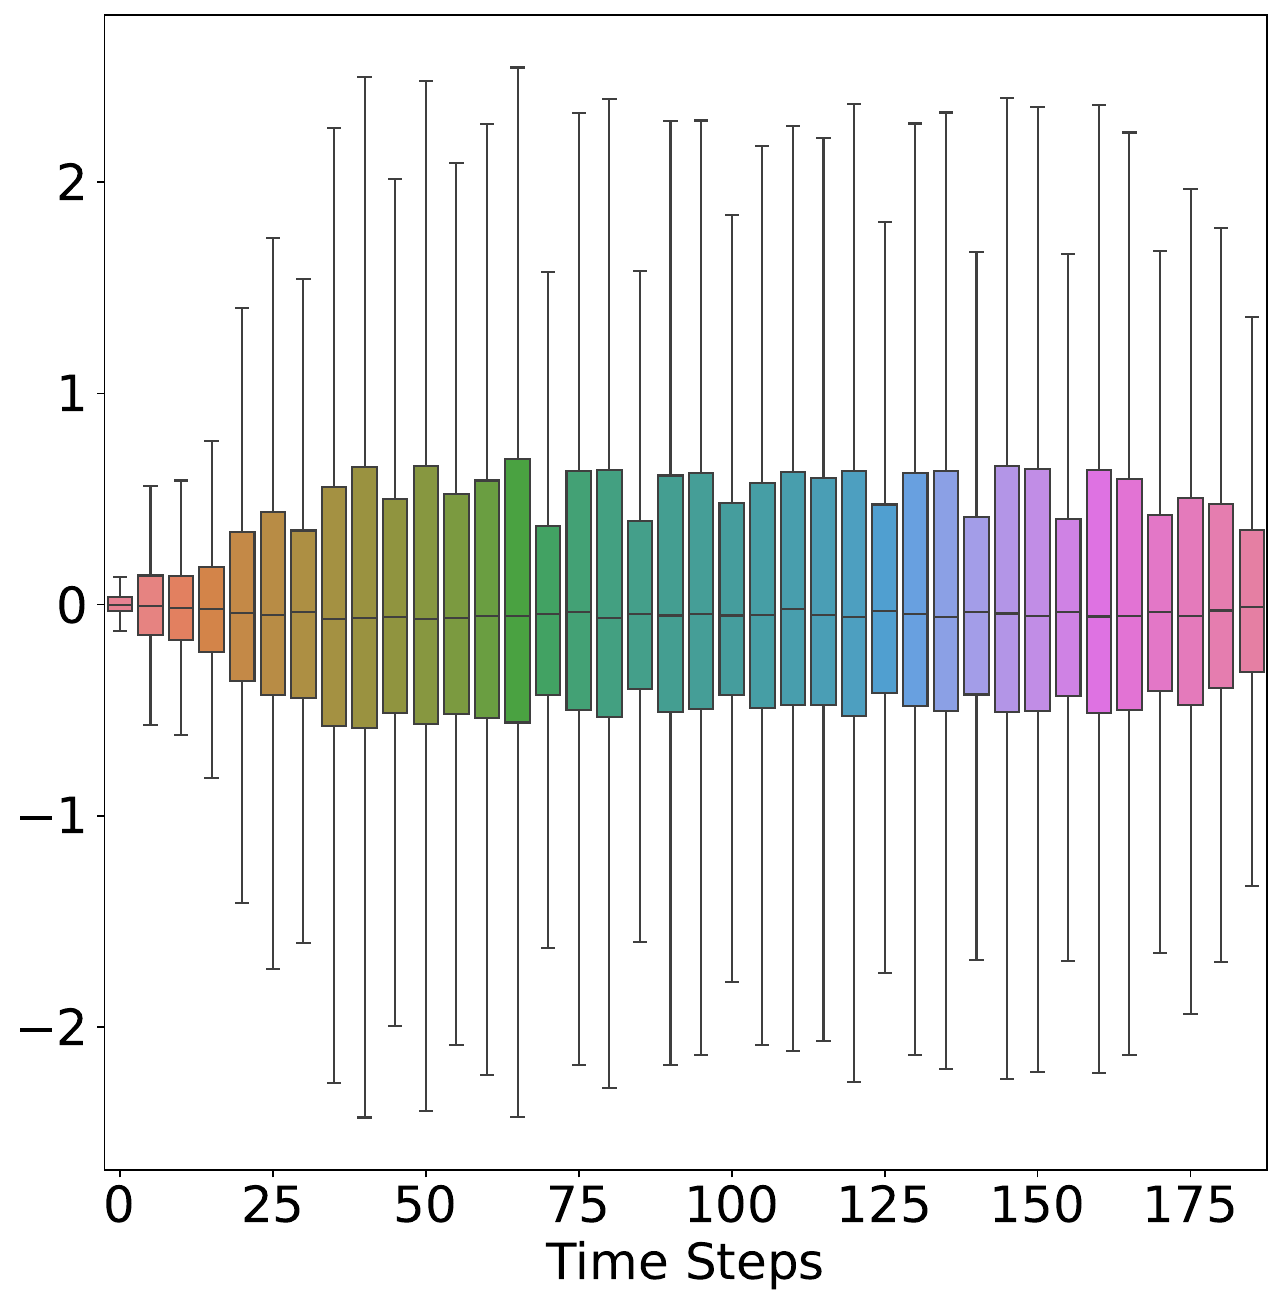}
    \end{minipage}
  }\hfill %\hspace{0.01\textwidth}
  \subcaptionbox{Uniform quantization on $\overline{A}_t$\label{observation:vmamba:s:deltaA_hist}}{
    \begin{minipage}{0.235\linewidth}
      \centering
      \includegraphics[width=\linewidth]{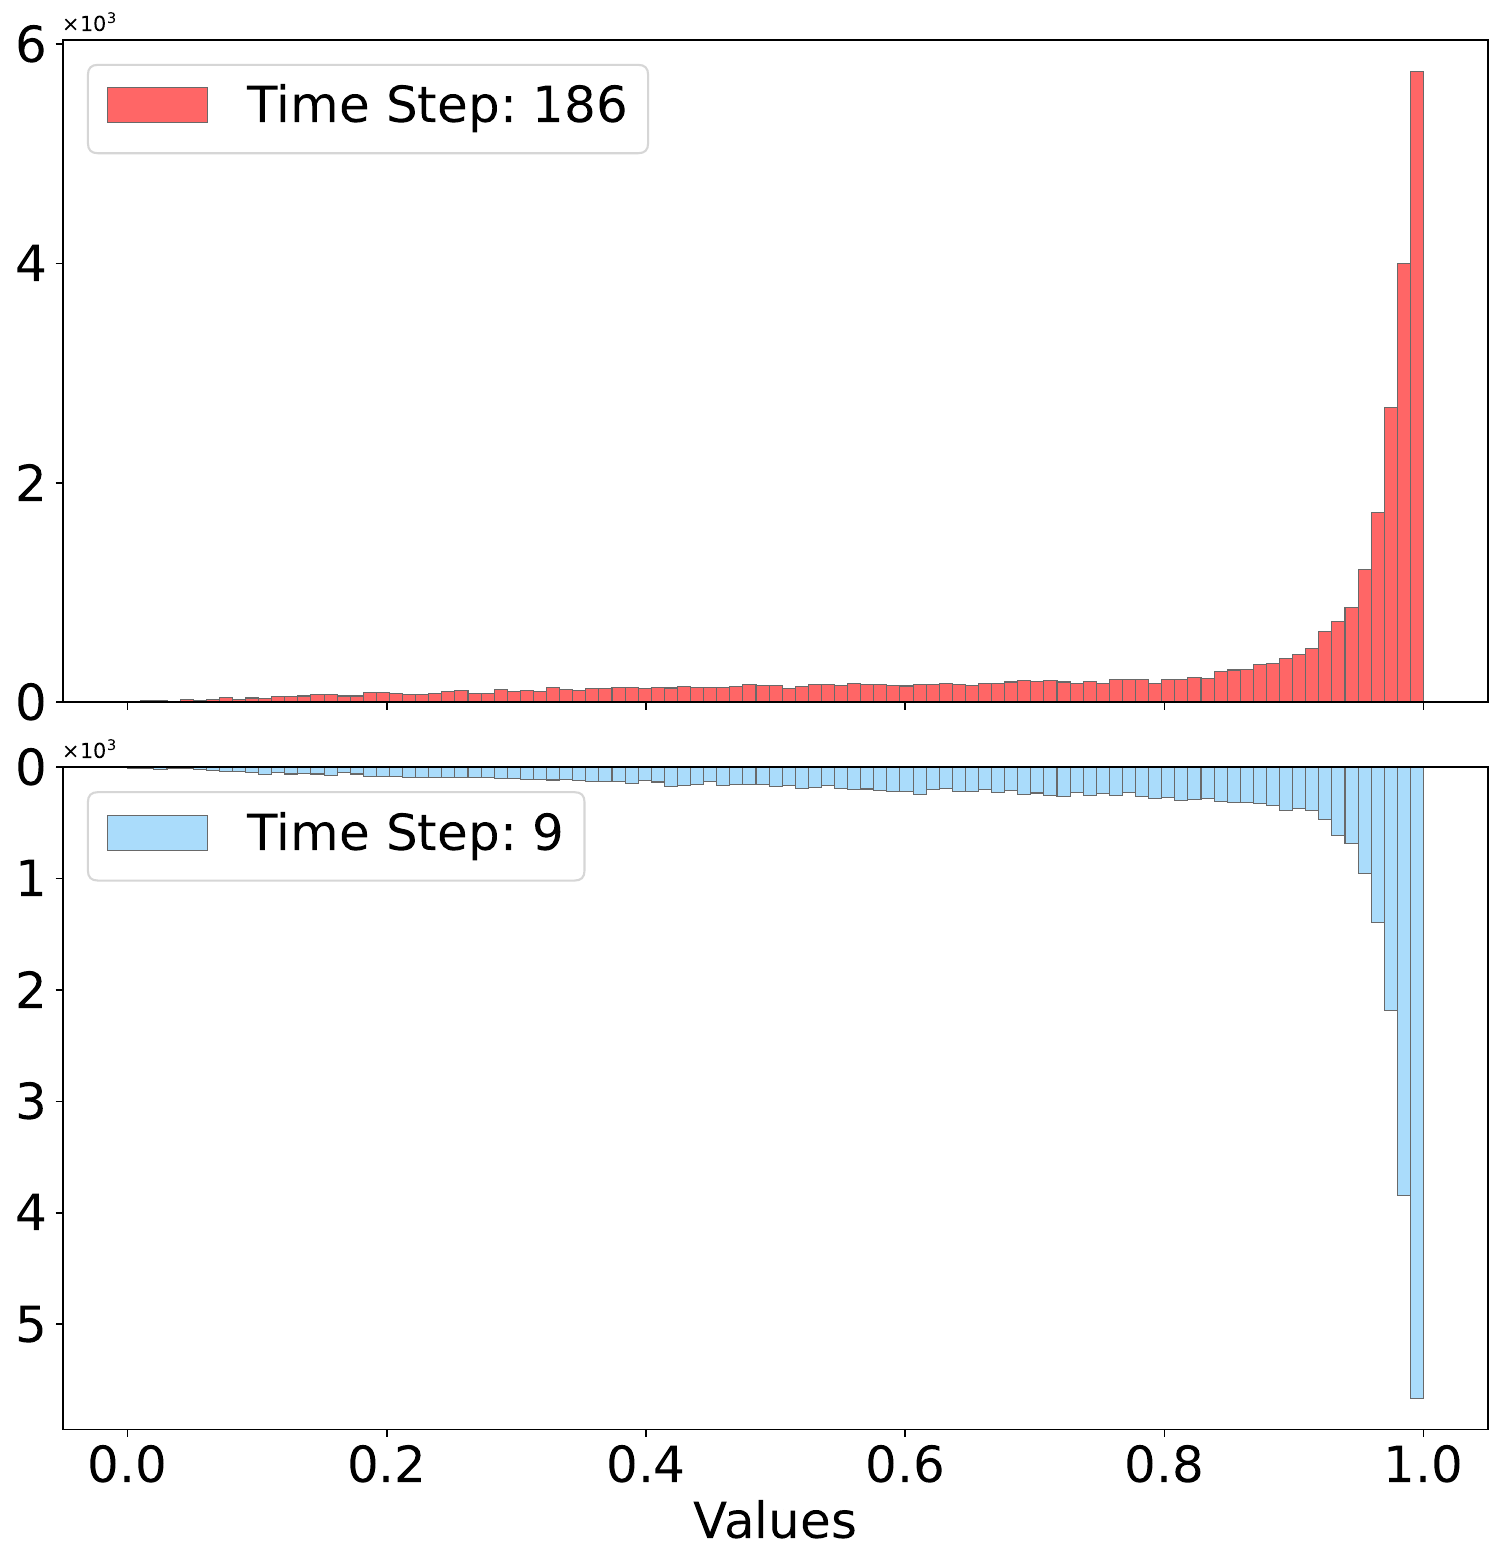}
    \end{minipage}
  }\hfill %\hspace{0.01\textwidth}
  \subcaptionbox{Uniform quantization on $h_t$\label{observation:vmamba:s:state_hist}}{
    \begin{minipage}{0.24\linewidth}
      \centering
      \includegraphics[width=\linewidth]{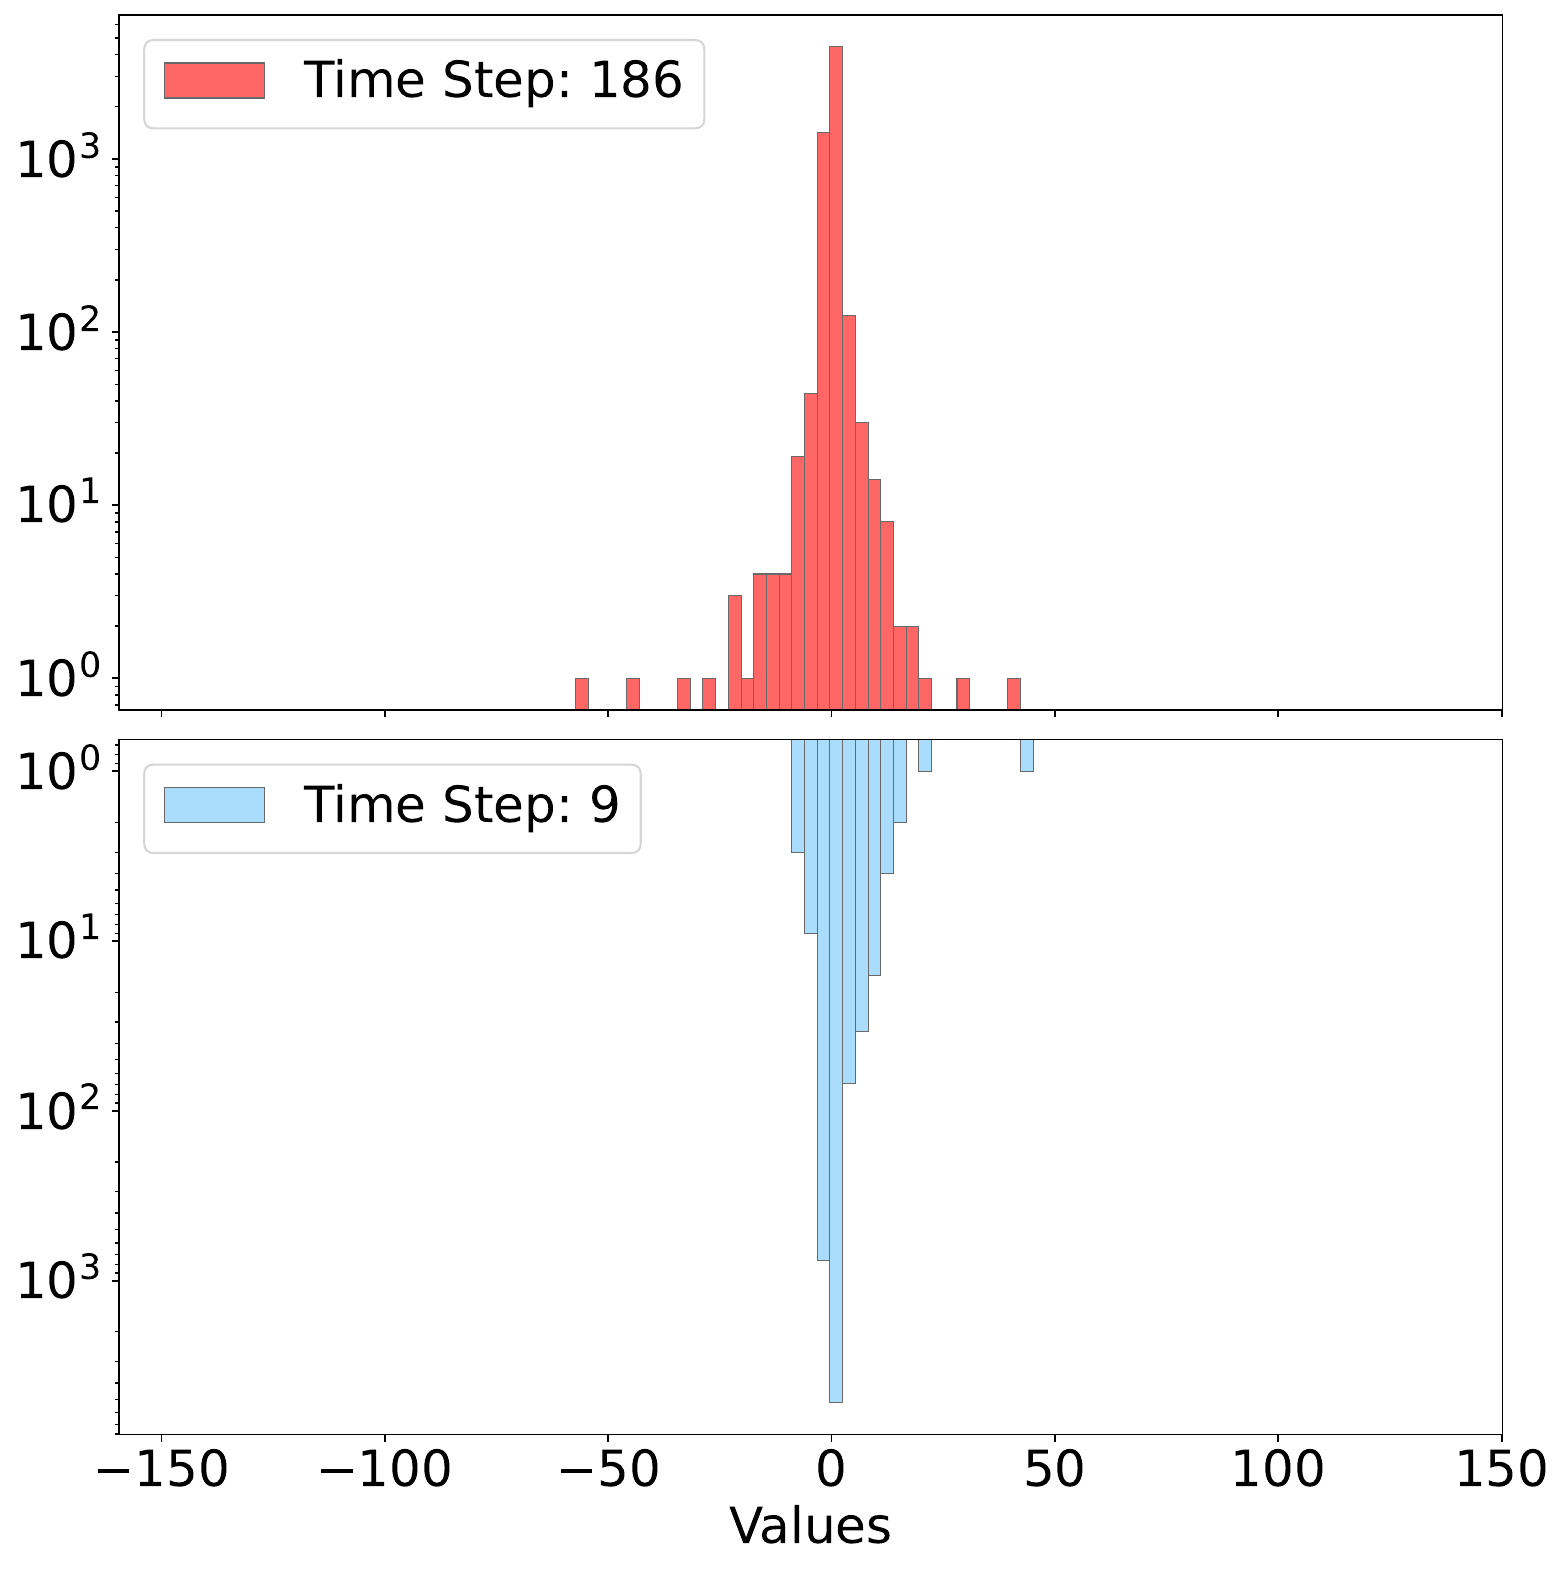}
    \end{minipage}
  }
  \caption{The statistics of discrete parameters $\overline{A}_t$ (15-th SSM) and hidden states $h_t$ (19-th SSM) are observed in the SSM of VMamba-S~\cite{vim}. We visualize $\overline{A}_t$ and $h_t$ at every fifth time step in the sequence, and the outliers in the boxplot of $h_t$ are omitted for better visualization. The horizontal axis of (a) and (b) presents observations across different time steps.}
  \label{observation:vmamba:s}
\end{figure*}
